# Supplementary material for: Learning Trajectory-Aware Transformer for Video Super-Resolution
Source: arXiv:2204.04216 source file (2022-04-20)

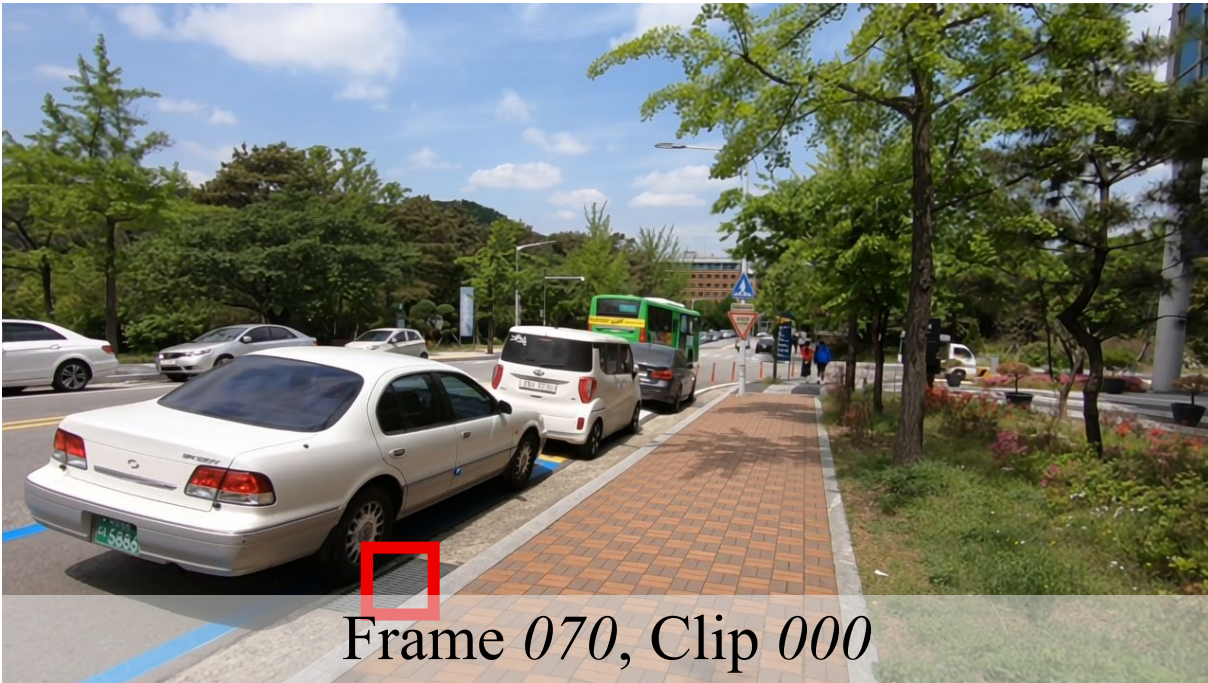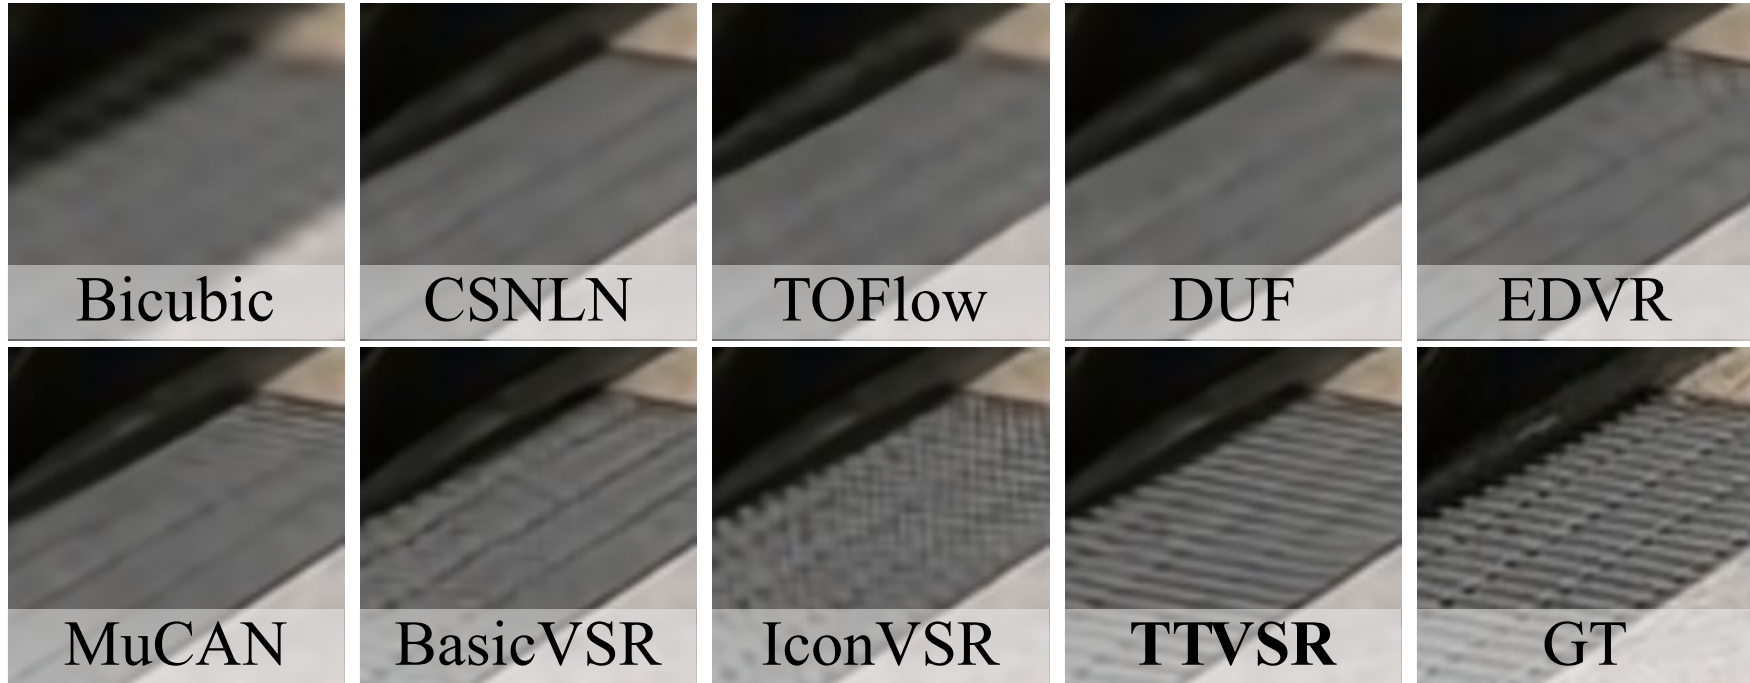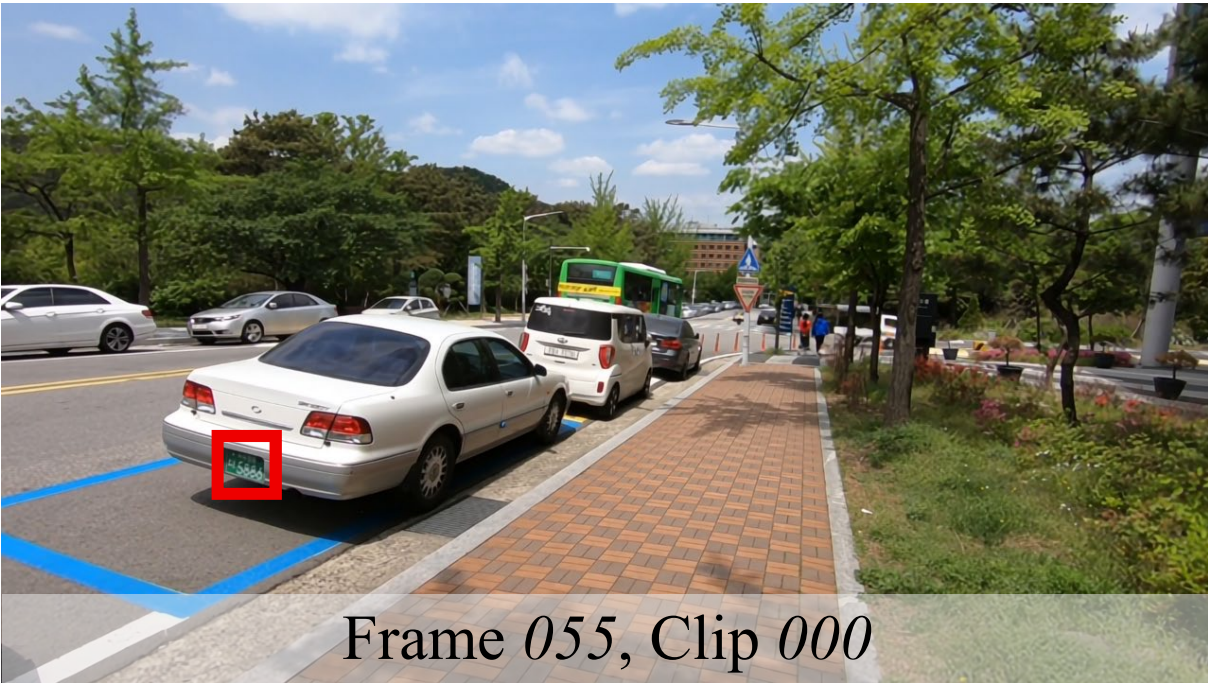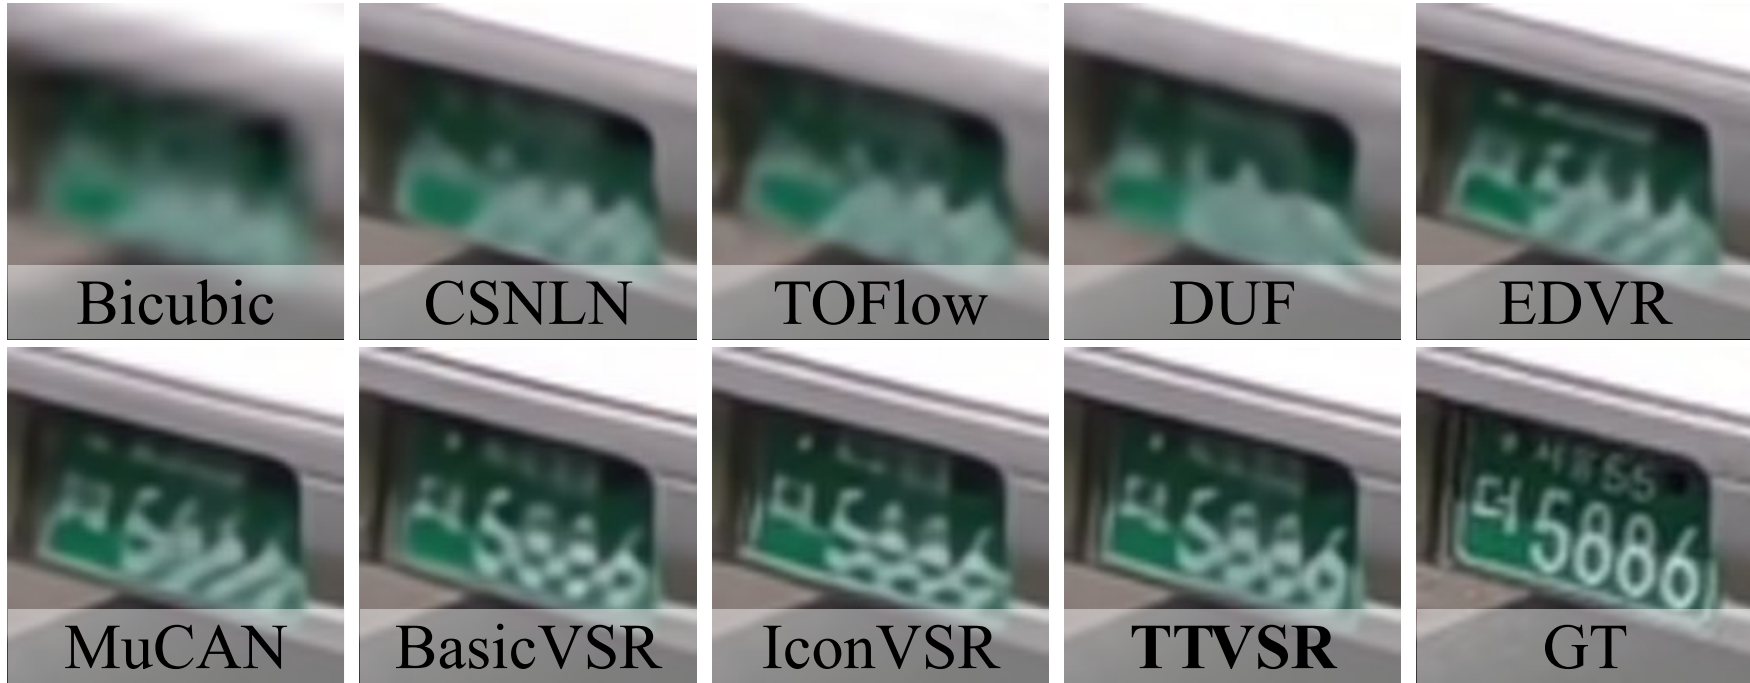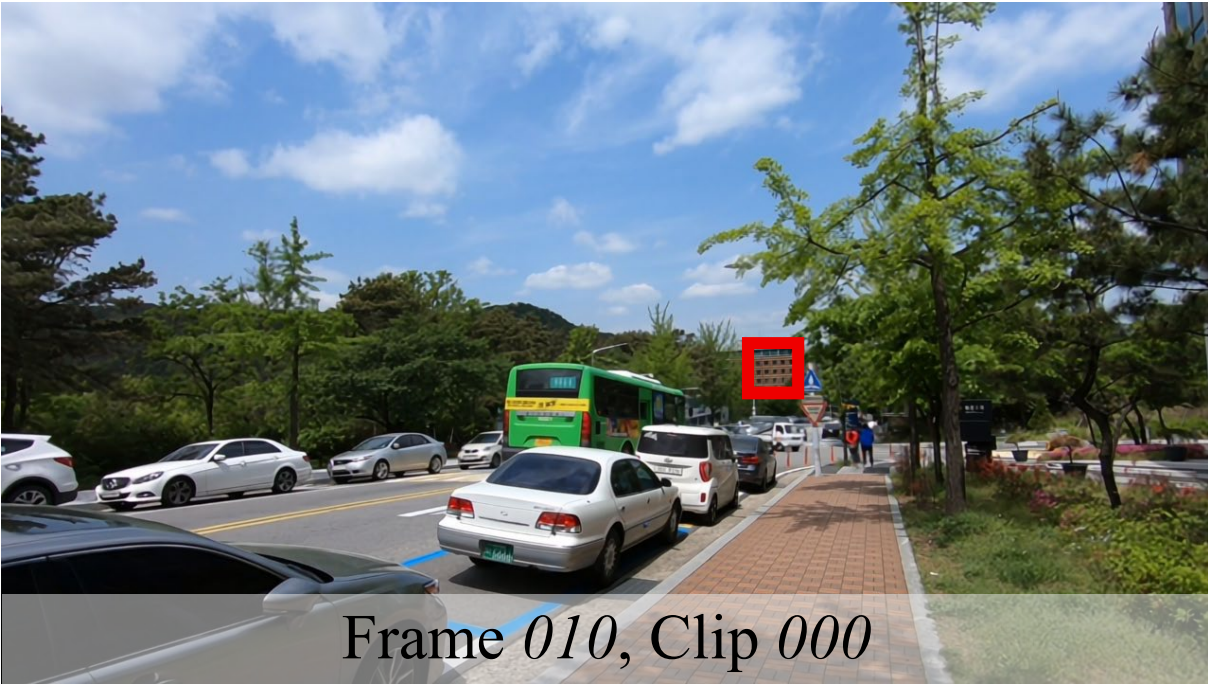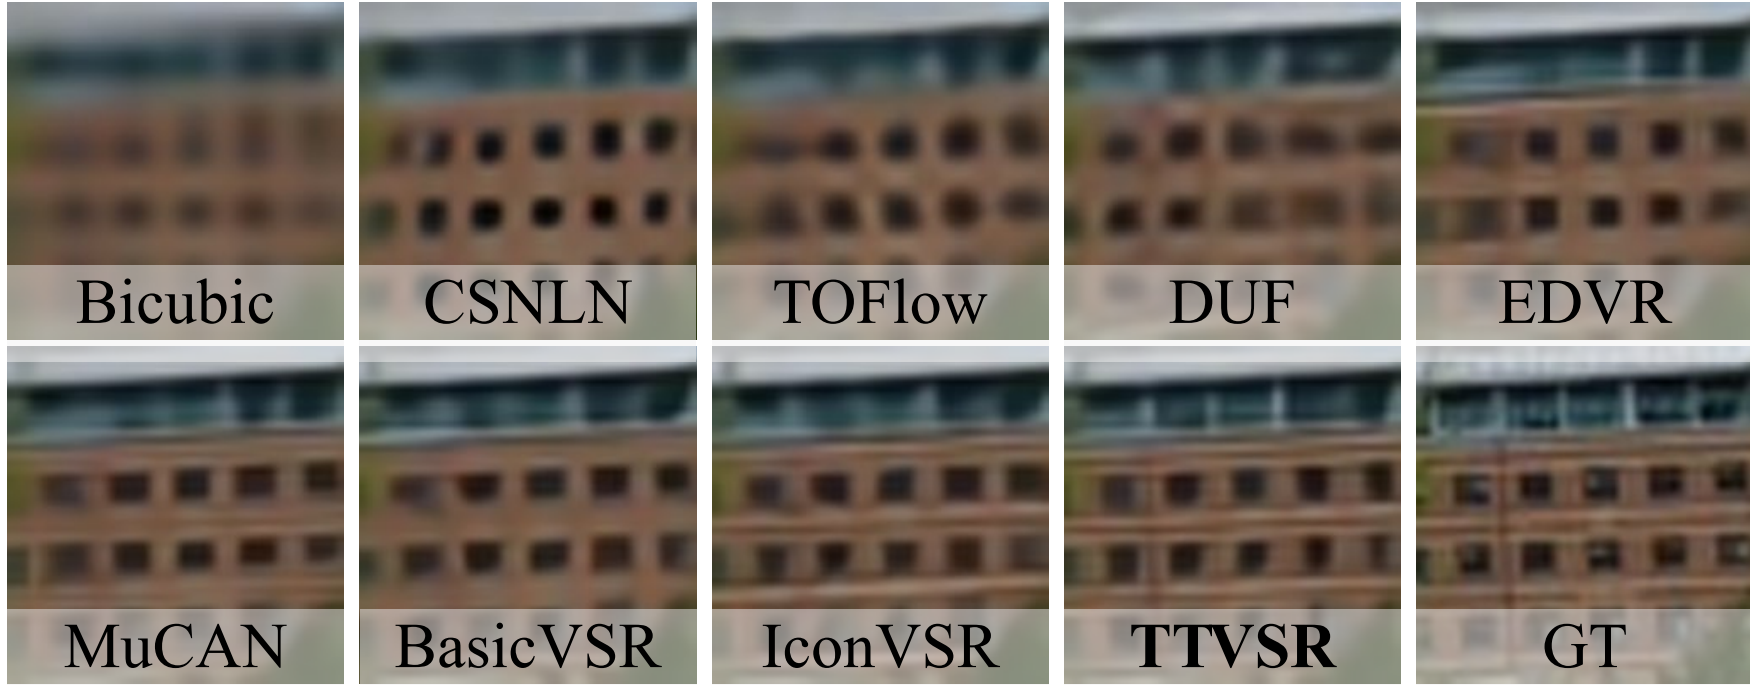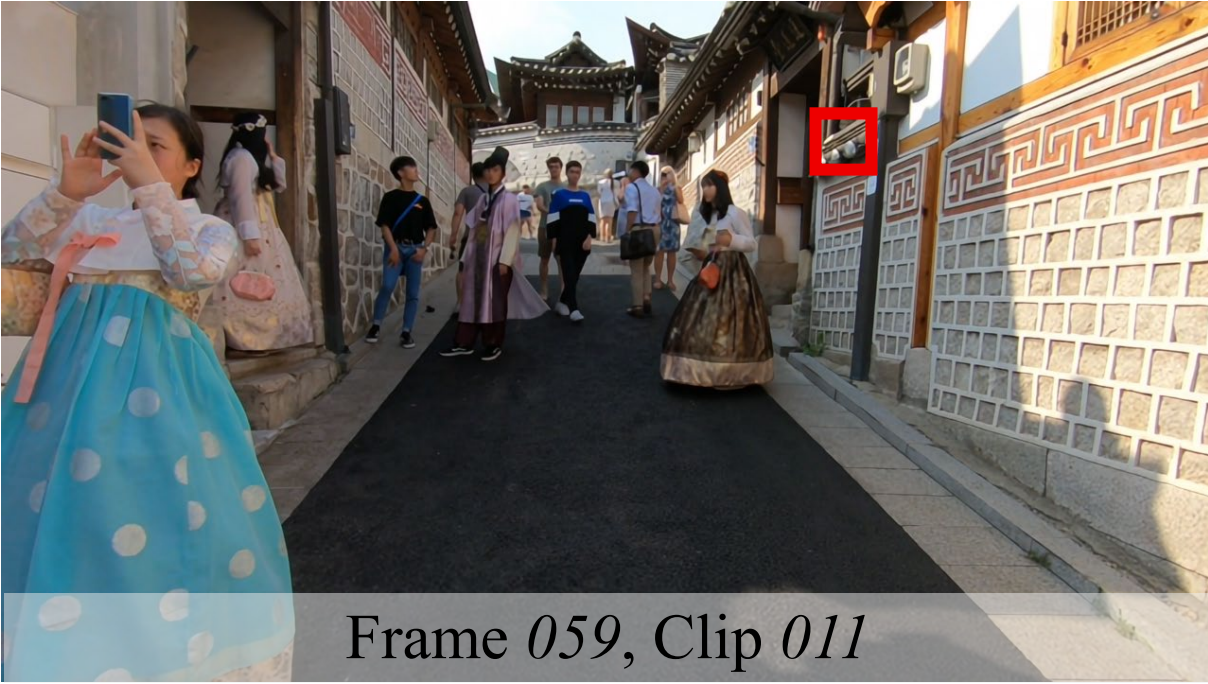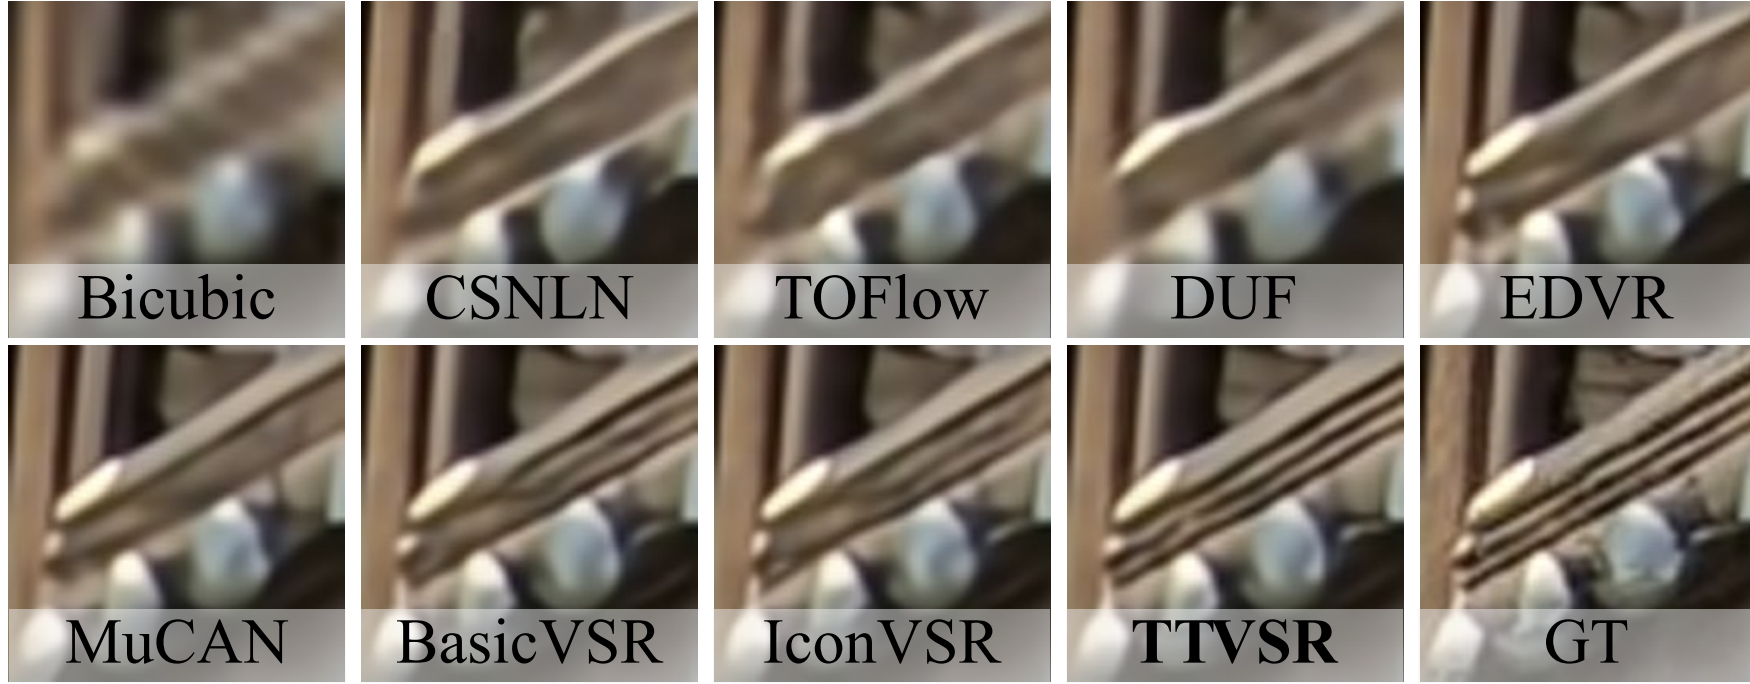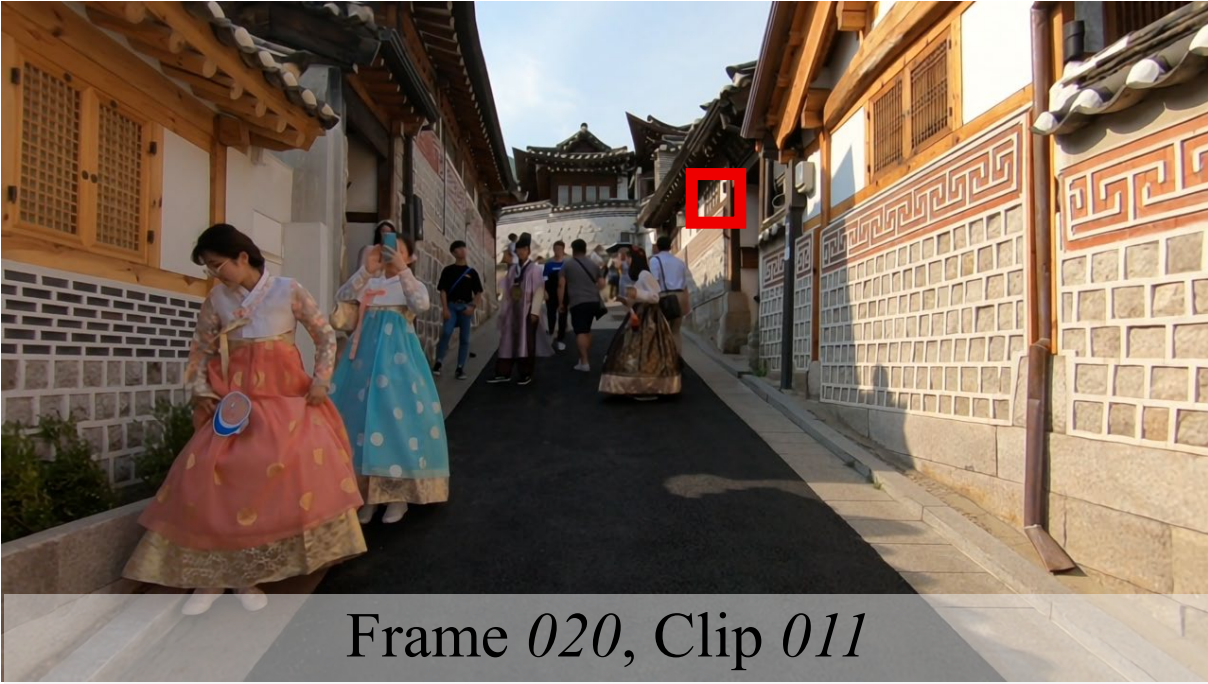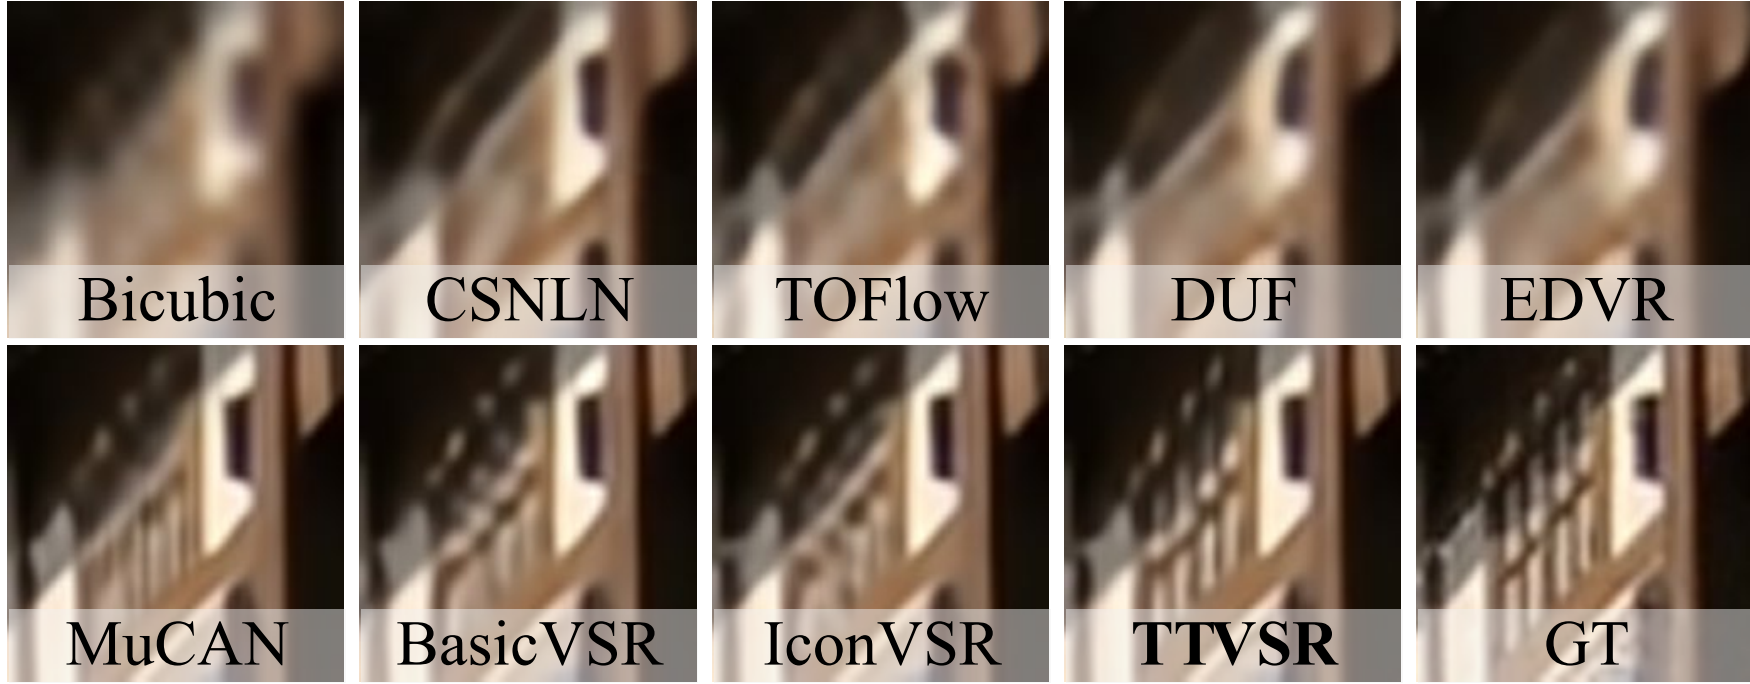



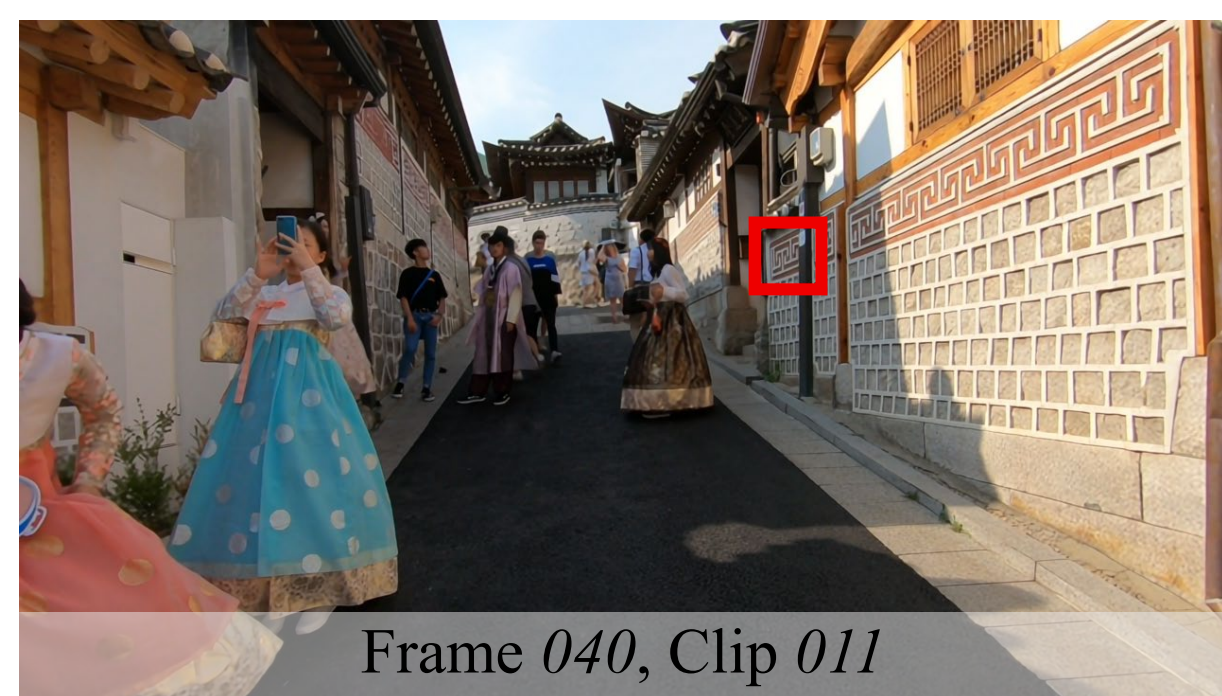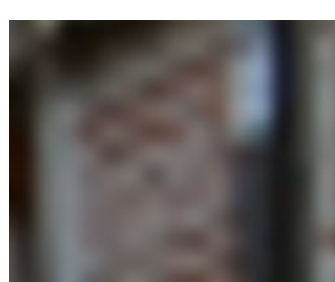

Bicubic

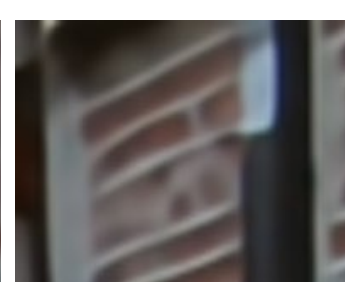

CSNLN

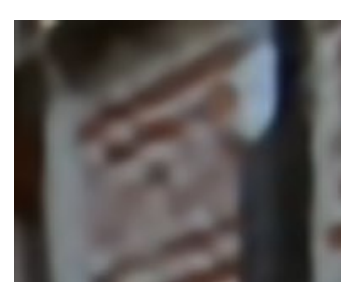

TOFlow

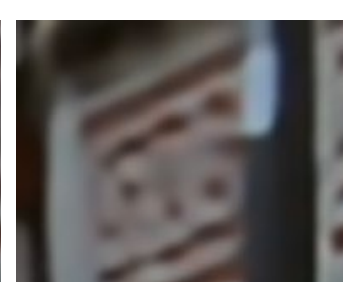

DUF

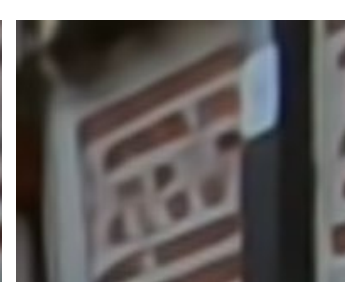

EDVR

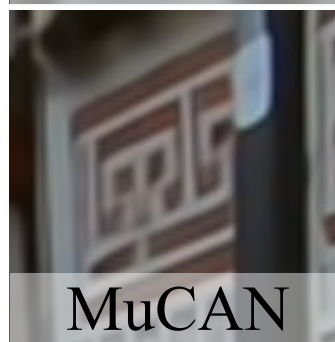

MuCAN

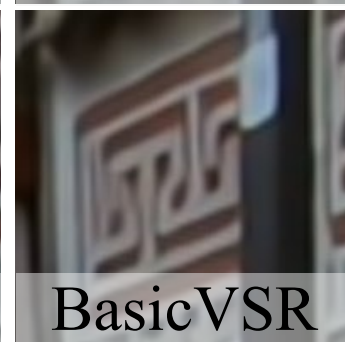

BasicVSR

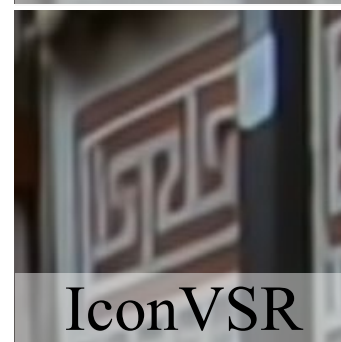

IconVSR

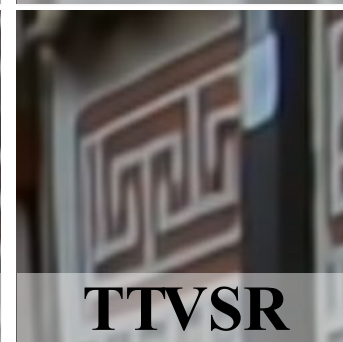

**TTVSR**

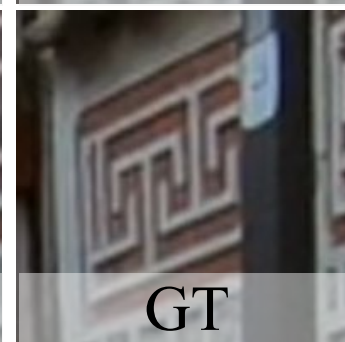

GT

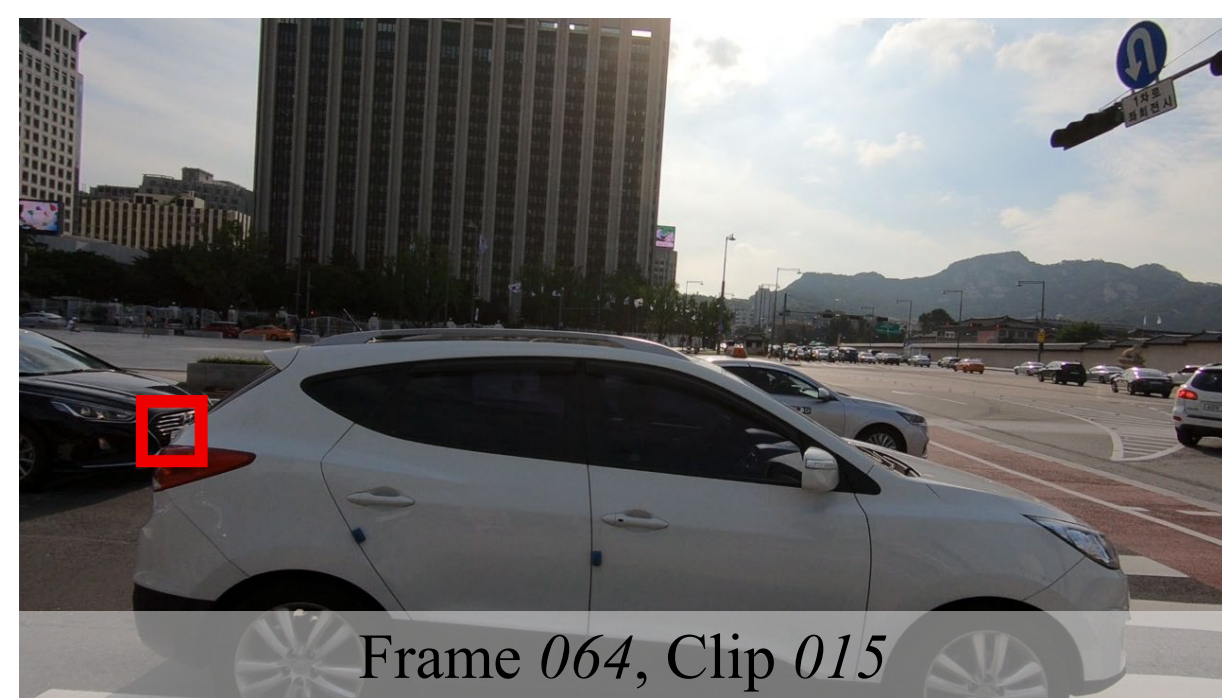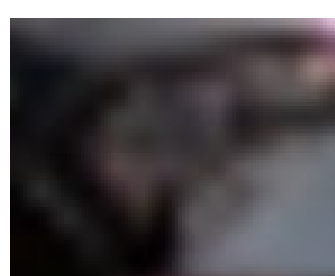

Bicubic

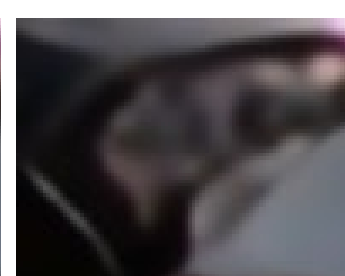

CSNLN

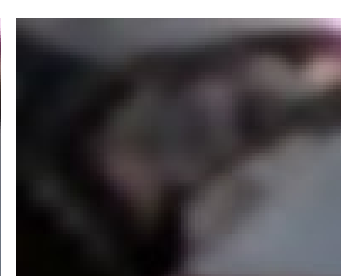

TOFlow

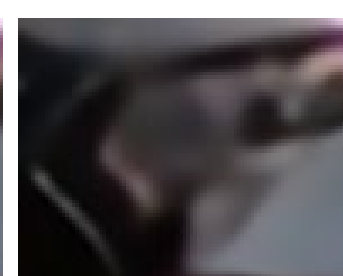

DUF

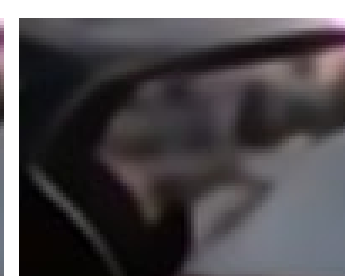

EDVR

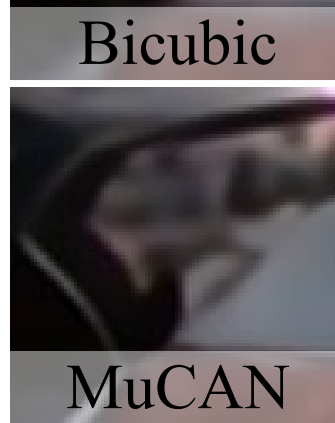

MuCAN

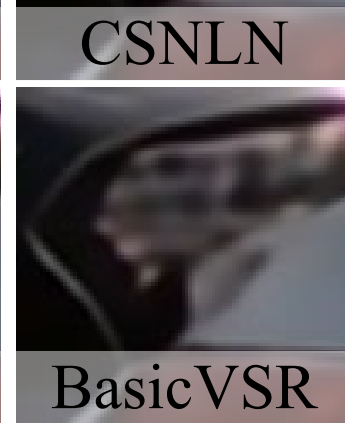

BasicVSR

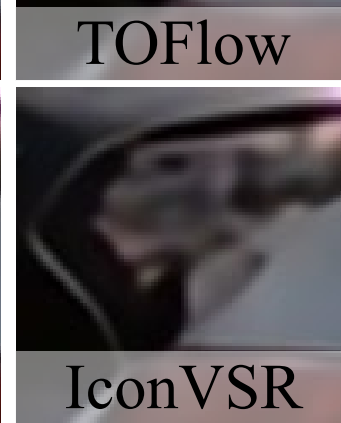

IconVSR

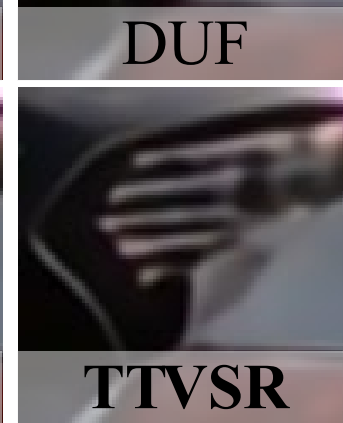

**TTVSR**

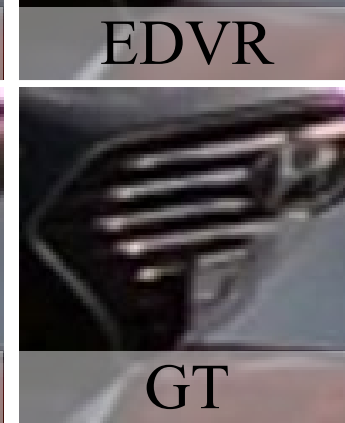

GT

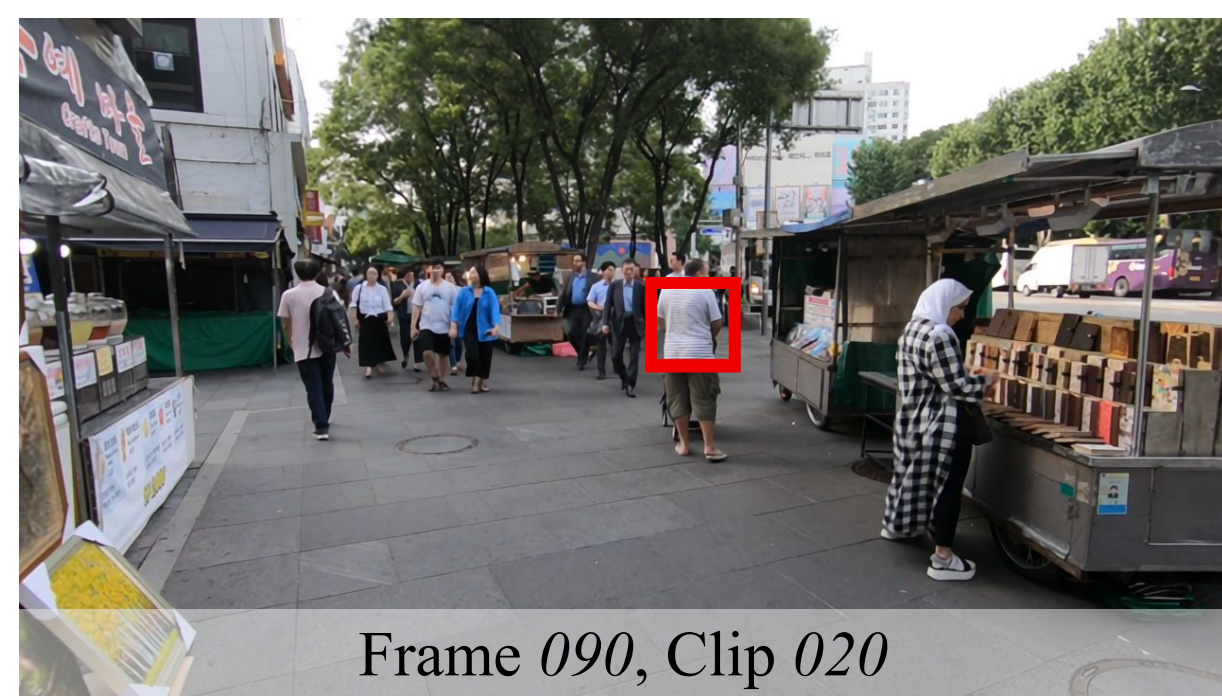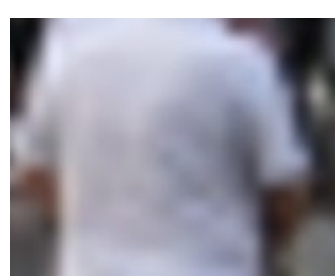

Bicubic

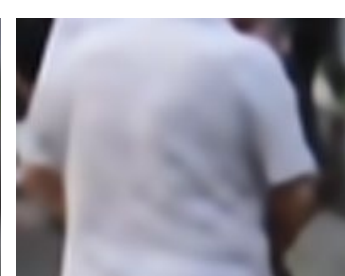

CSNLN

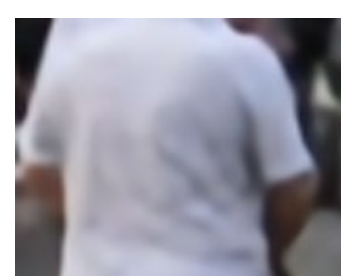

TOFlow

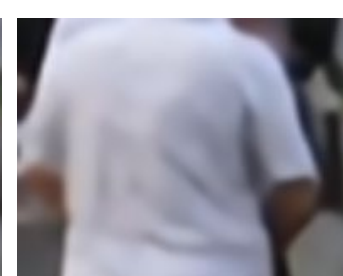

DUF

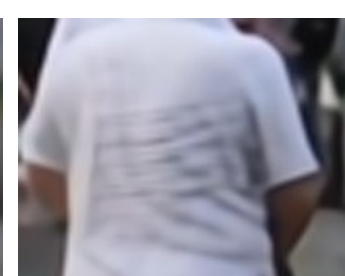

EDVR

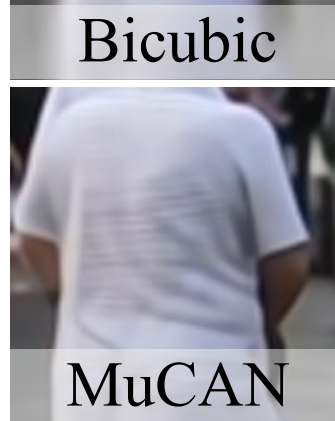

MuCAN

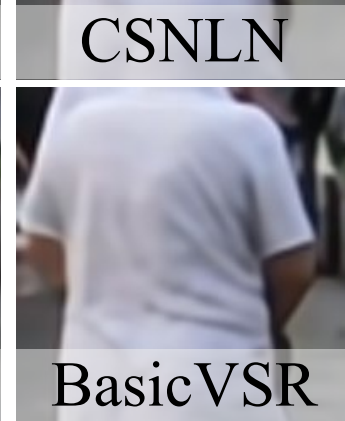

BasicVSR

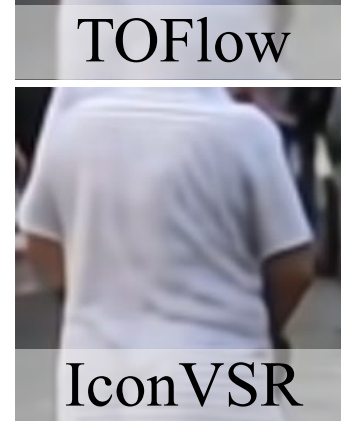

IconVSR

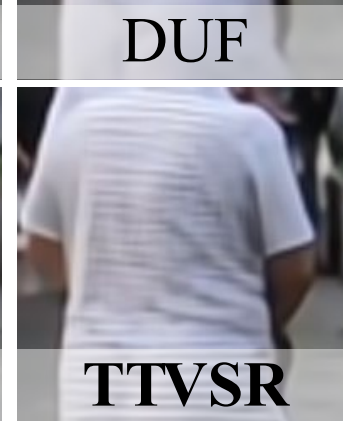

**TTVSR**

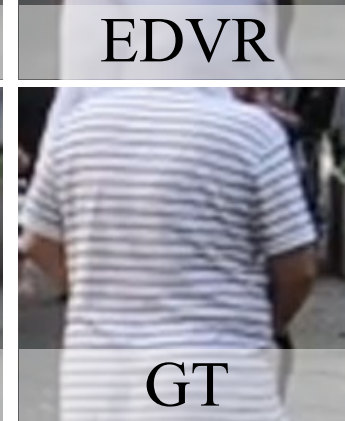

GT

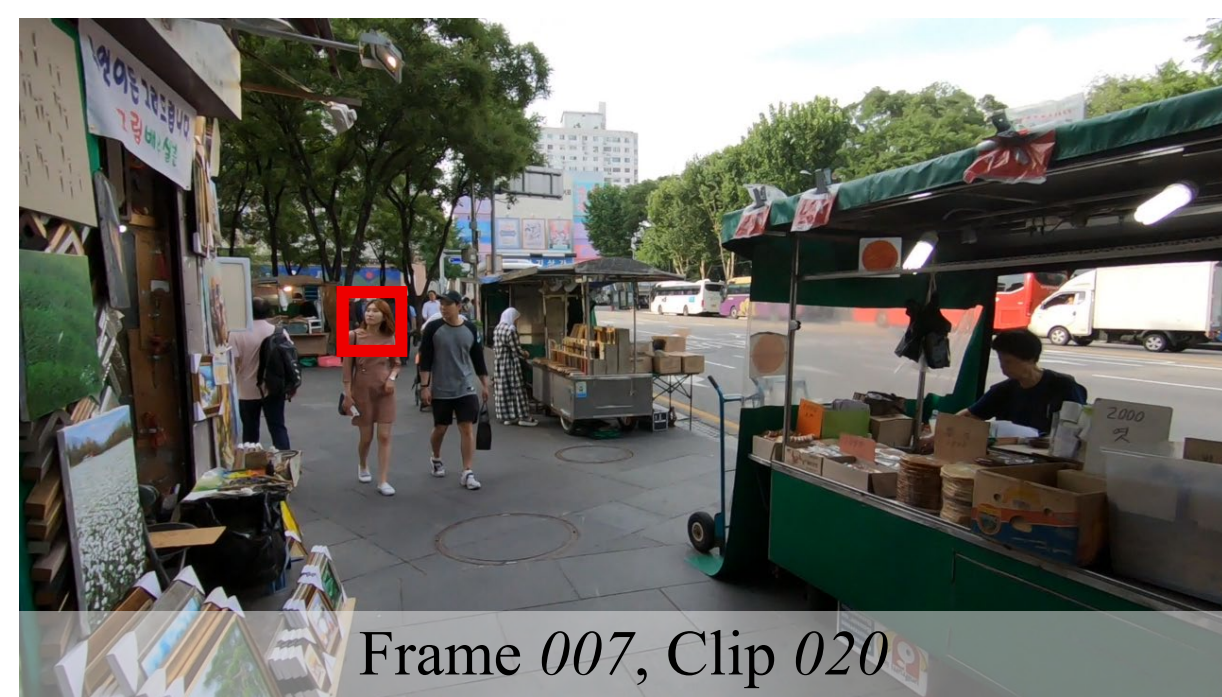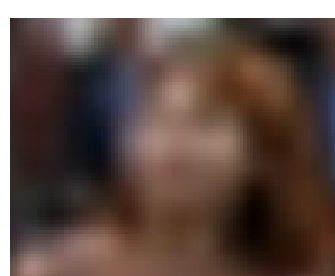

Bicubic

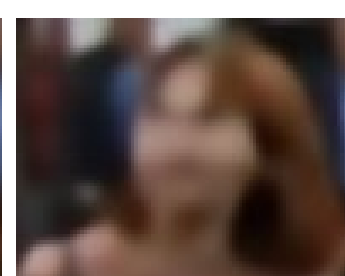

CSNLN

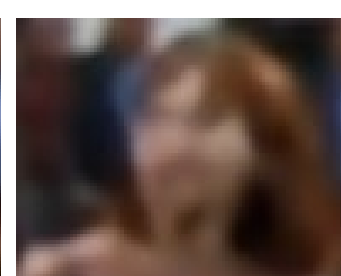

TOFlow

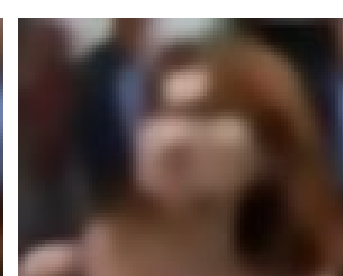

DUF

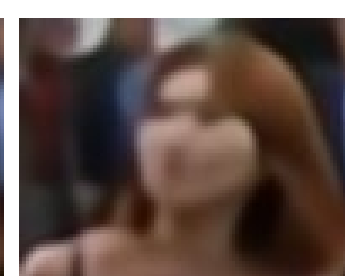

EDVR

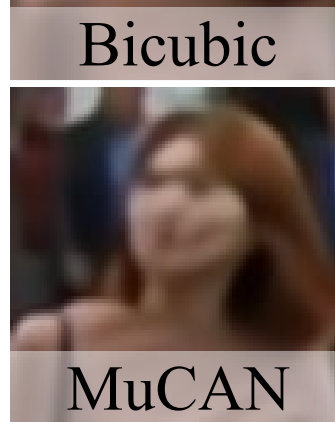

MuCAN

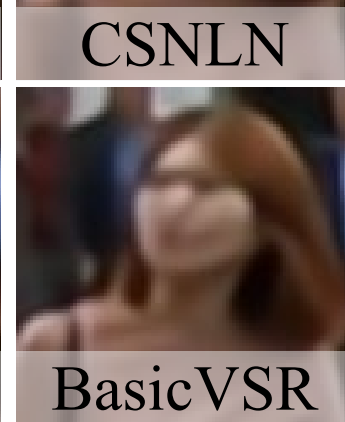

BasicVSR

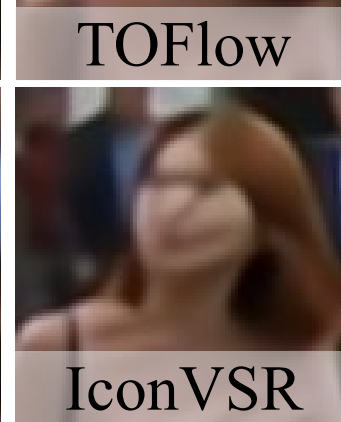

IconVSR

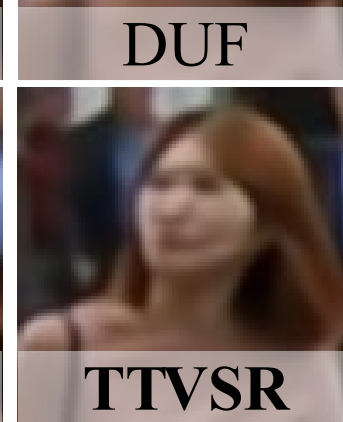

**TTVSR**

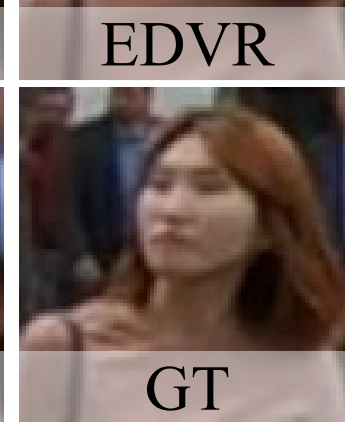

GT

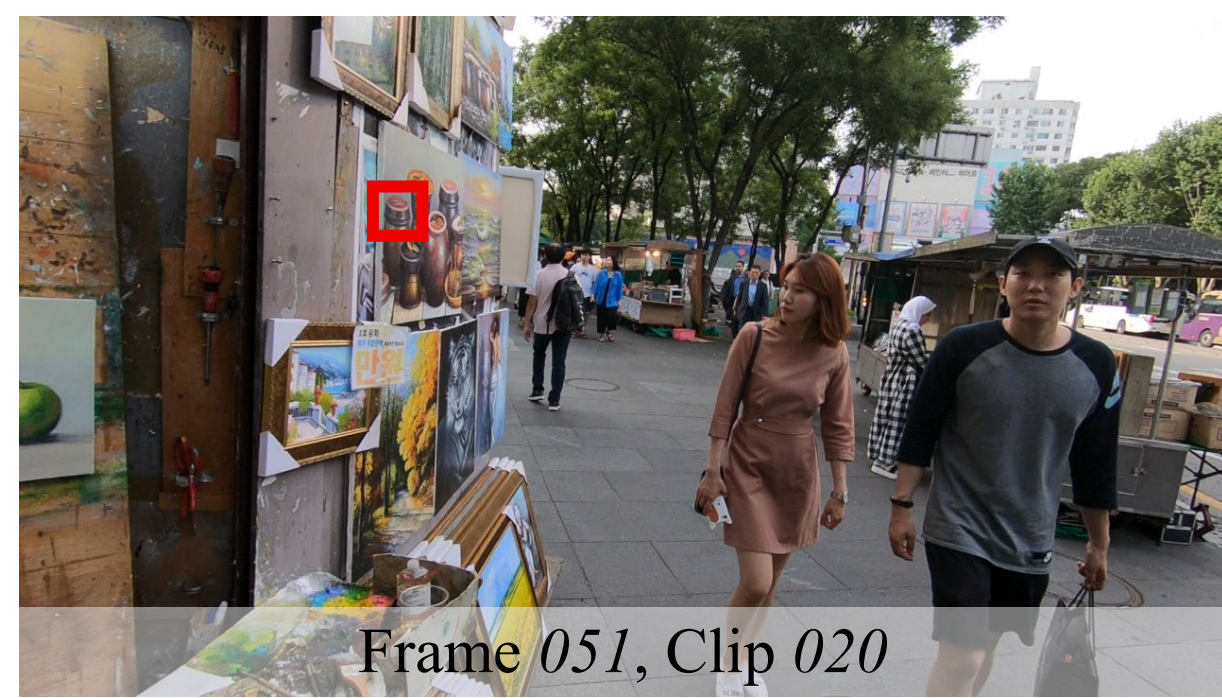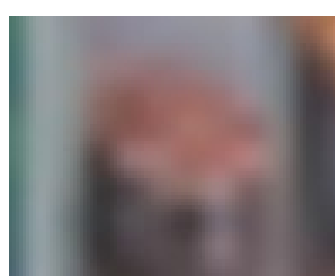

Bicubic

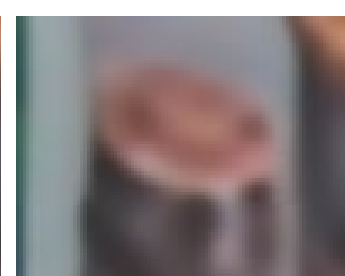

CSNLN

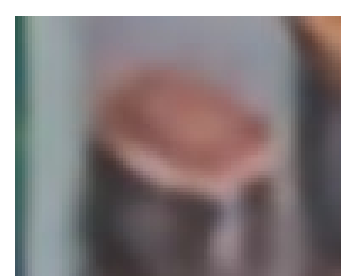

TOFlow

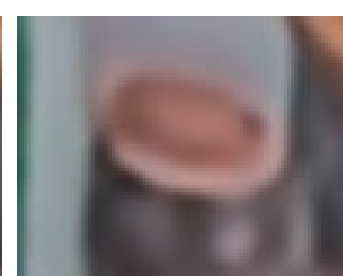

DUF

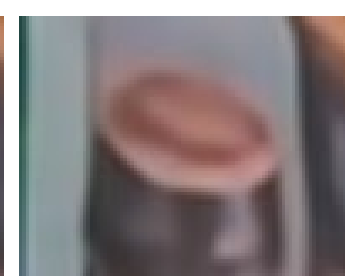

EDVR

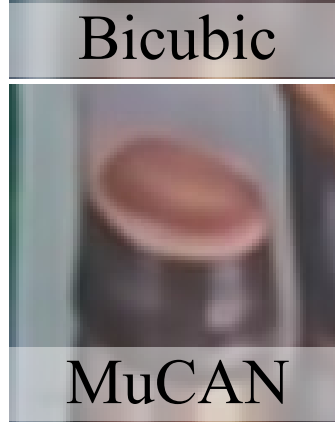

MuCAN

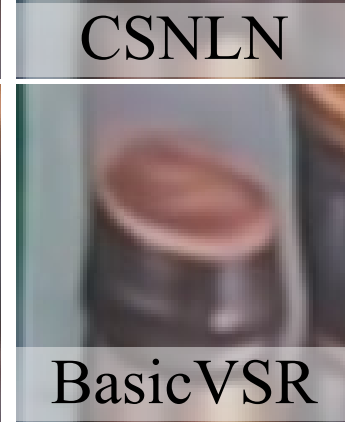

BasicVSR

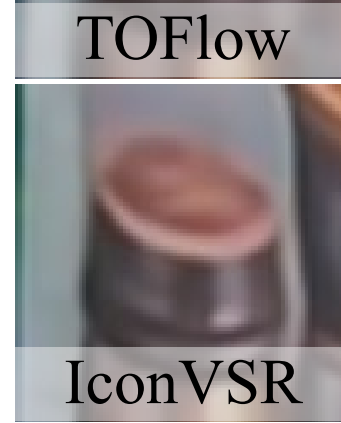

IconVSR

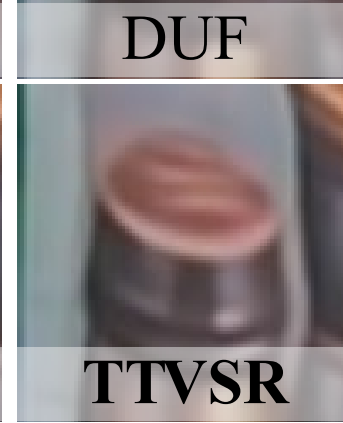

**TTVSR**

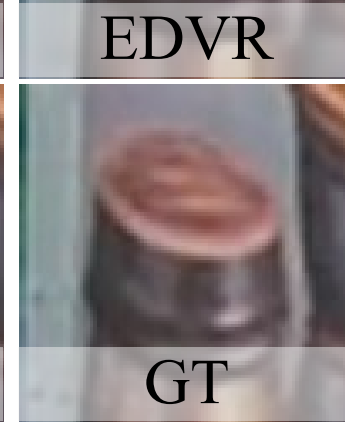

GT



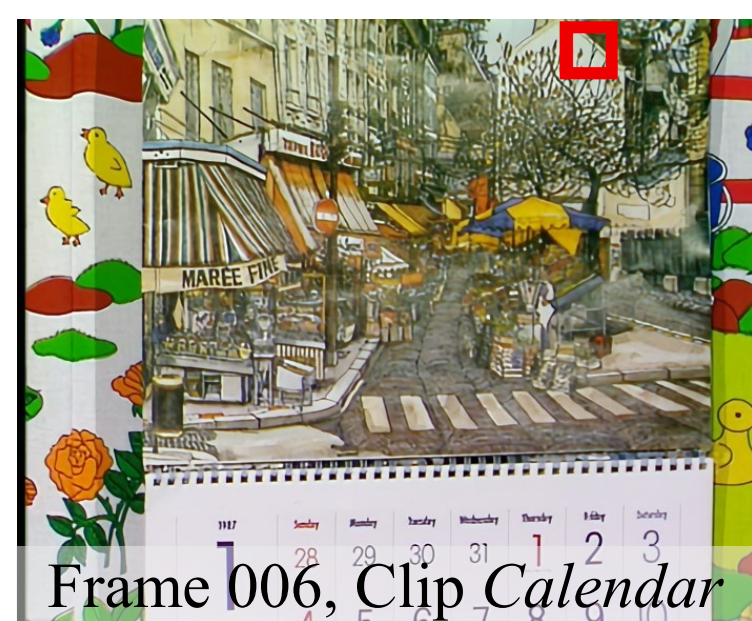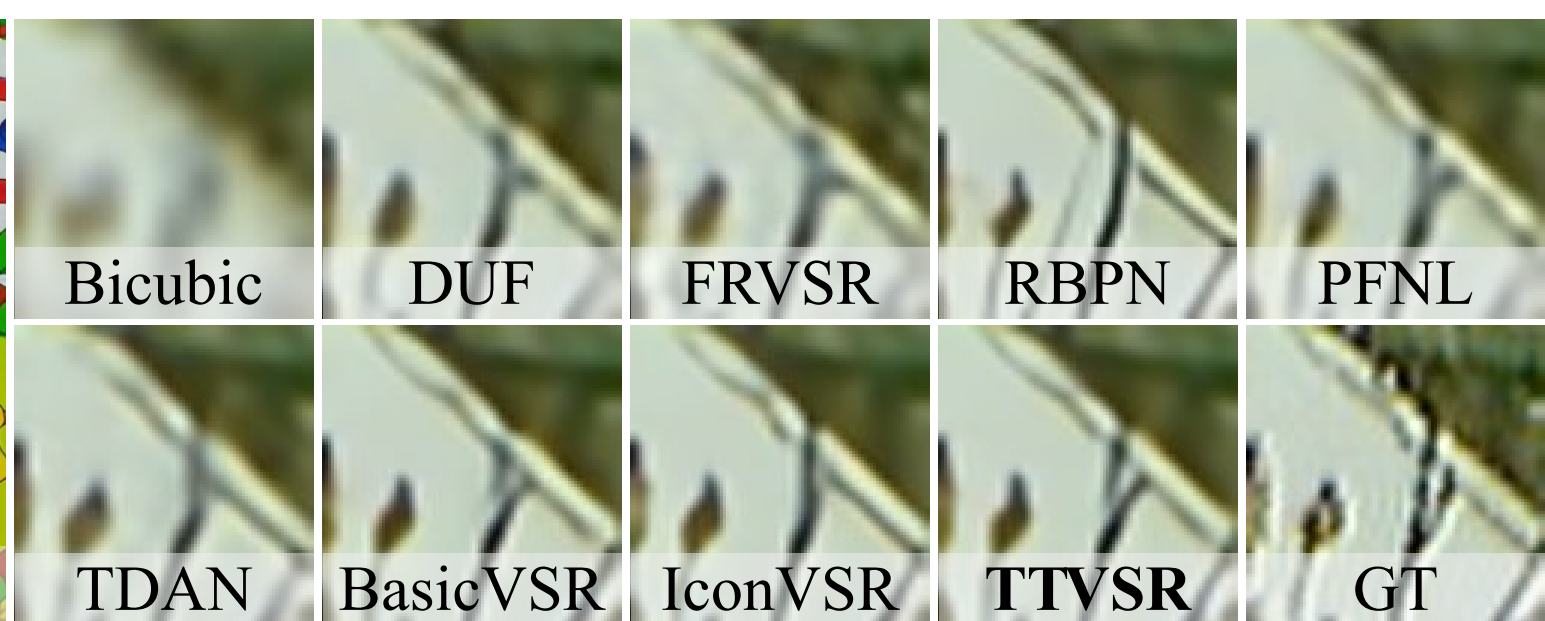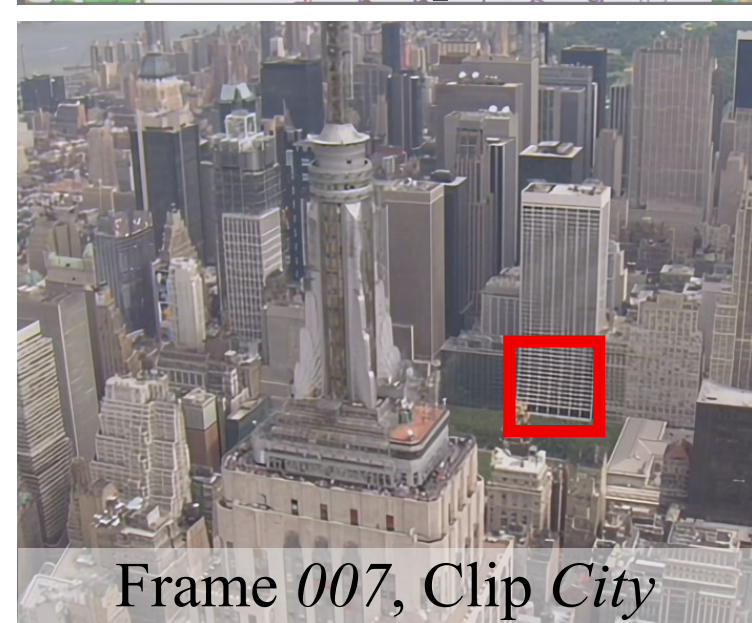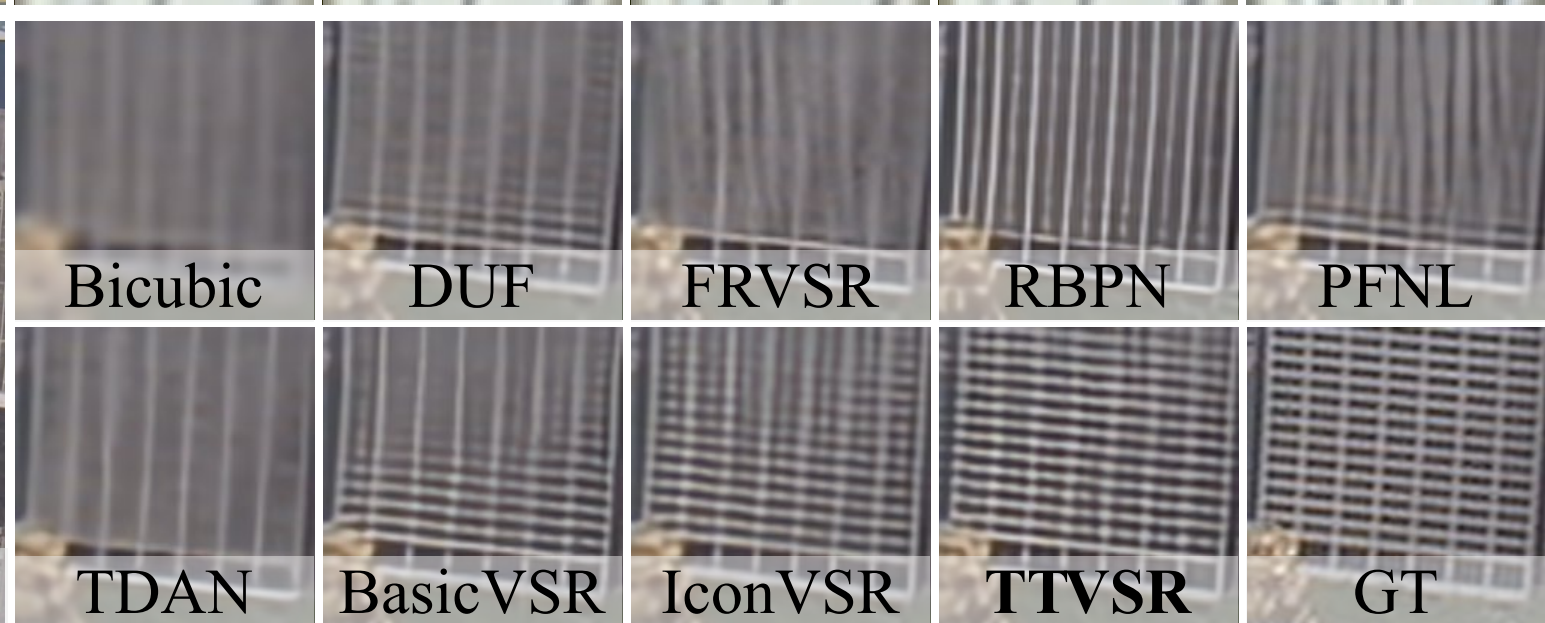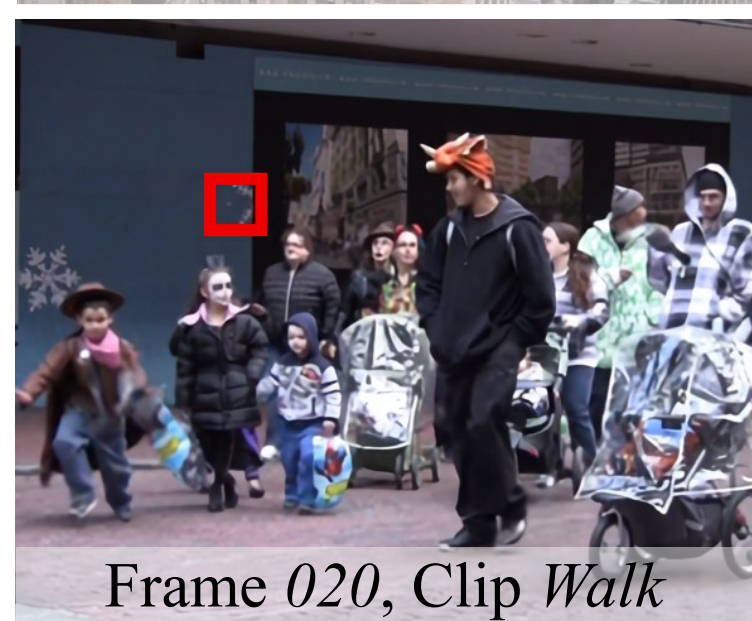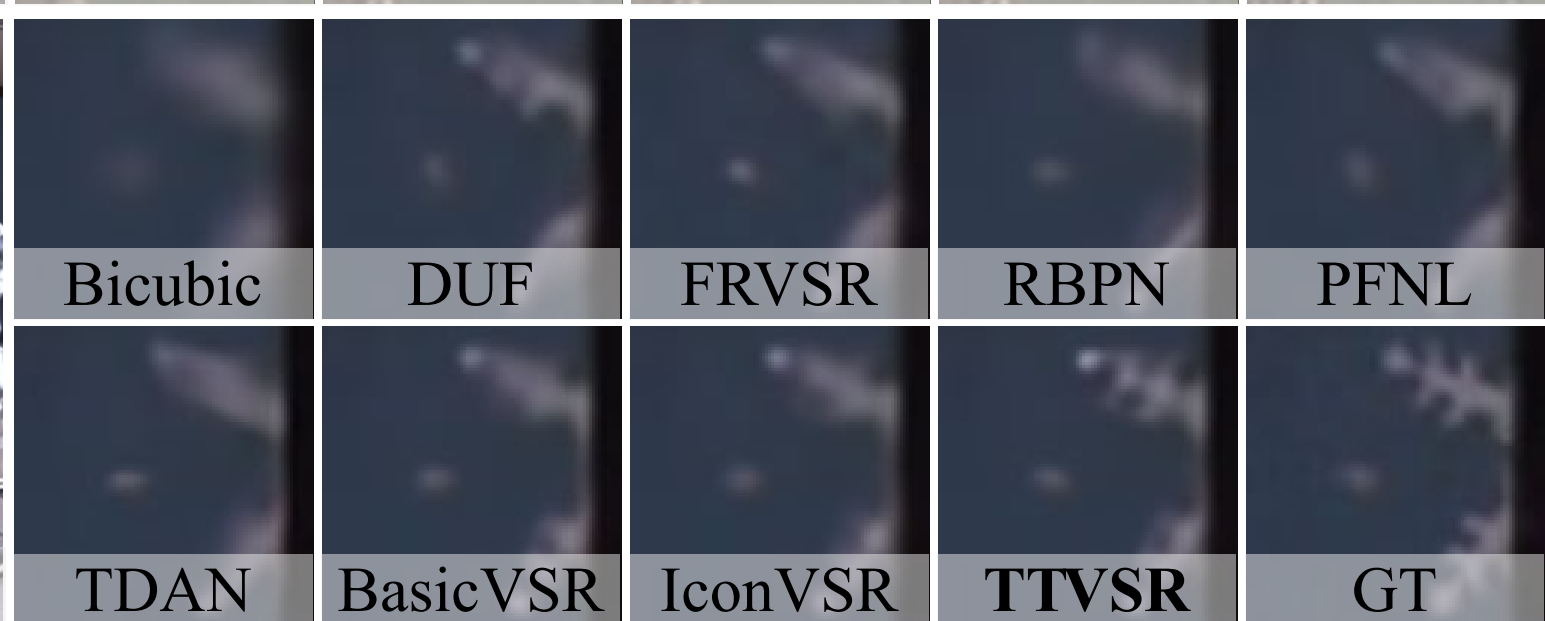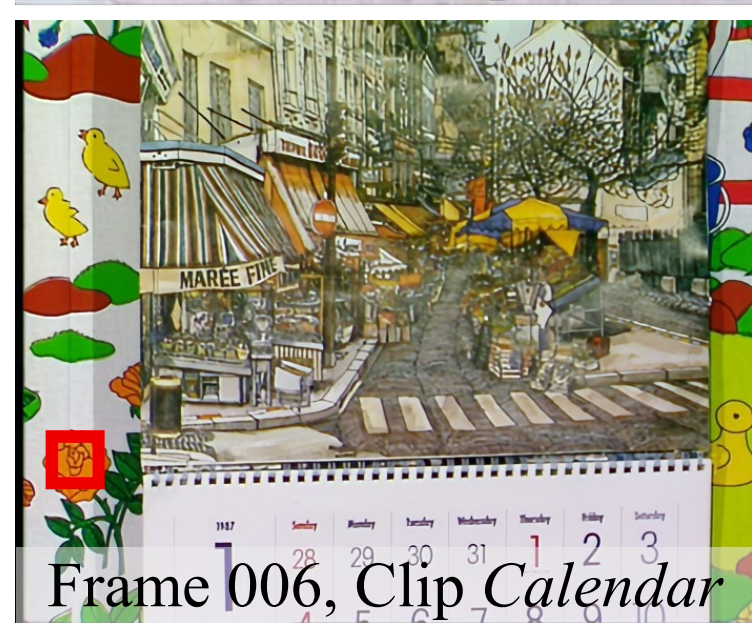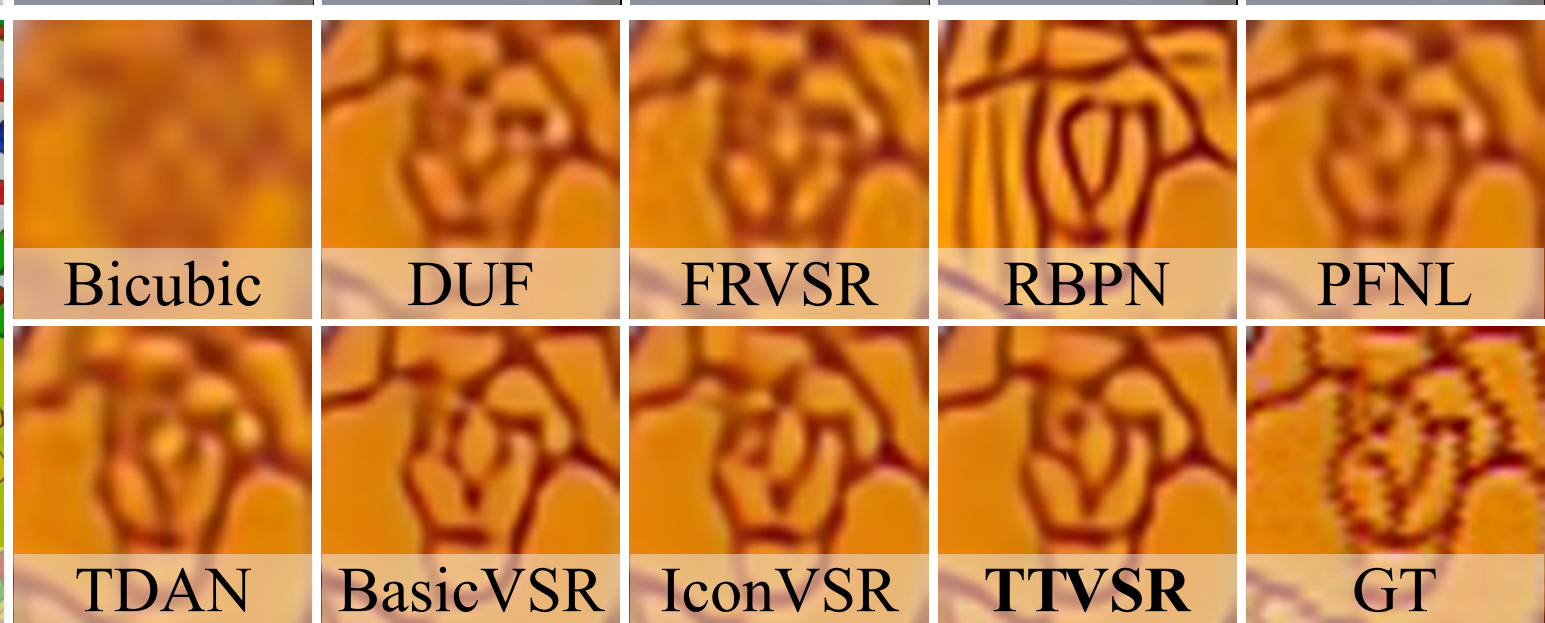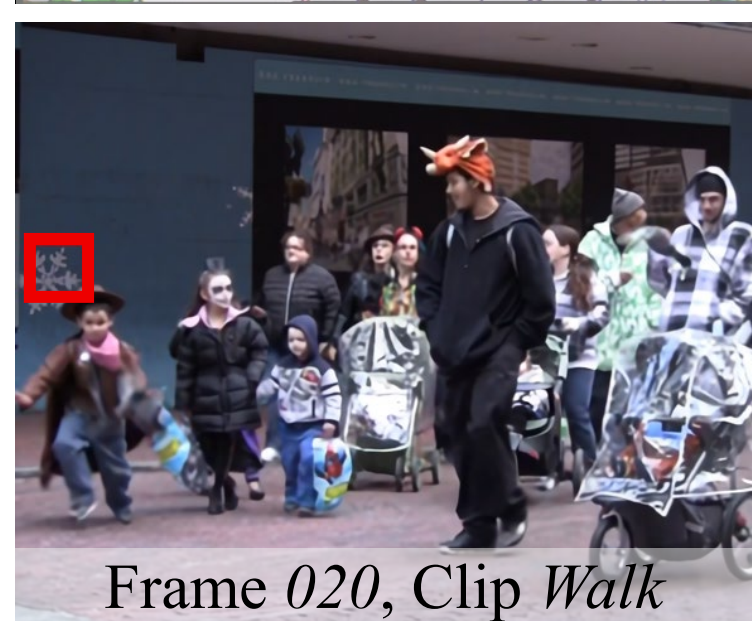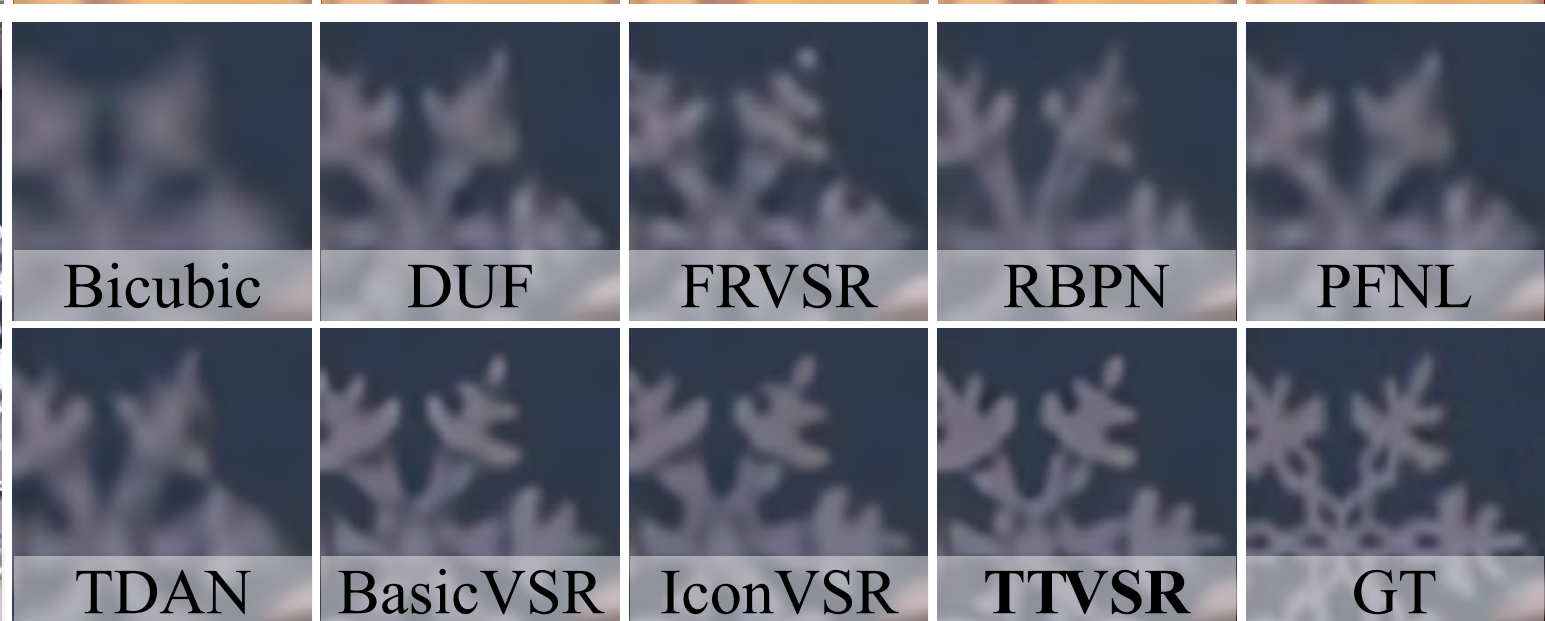



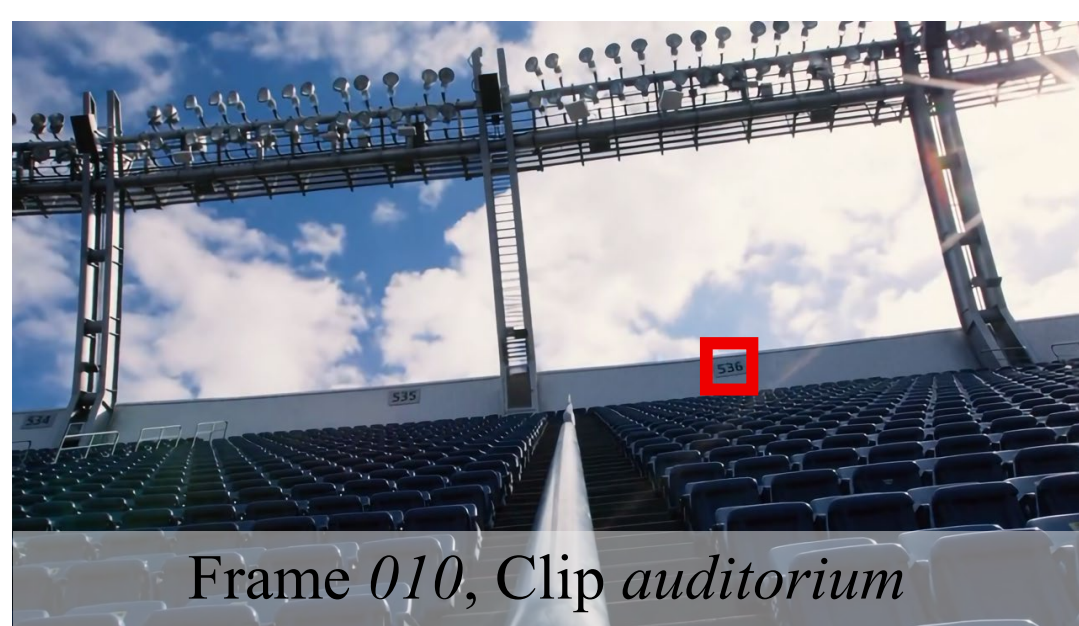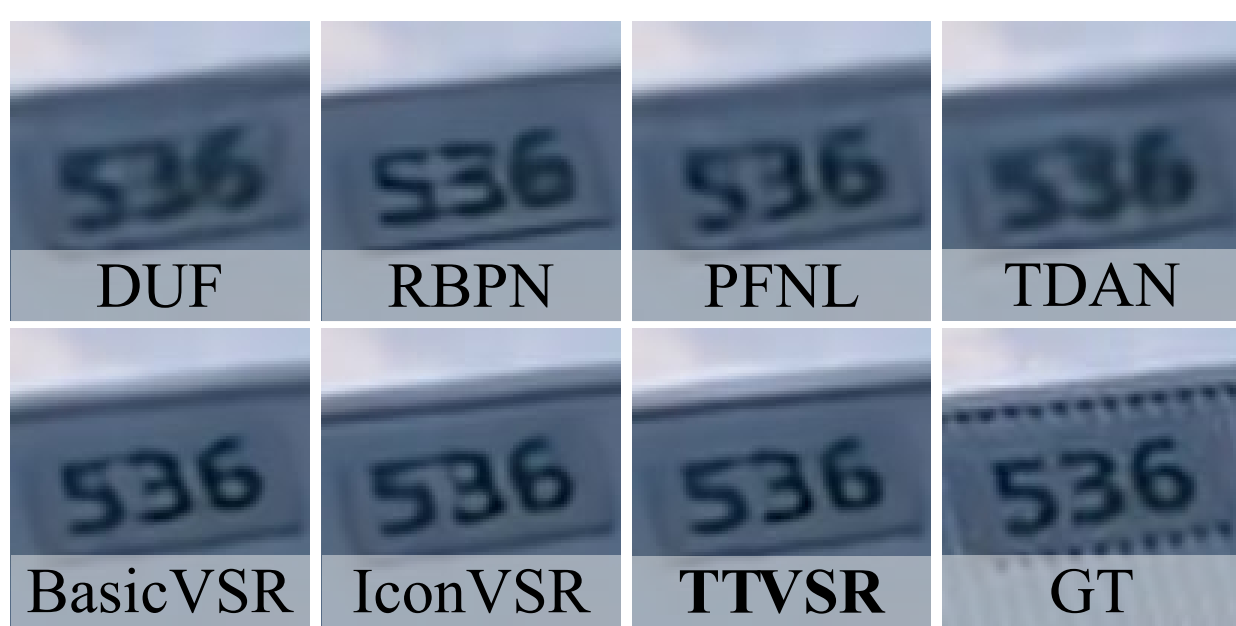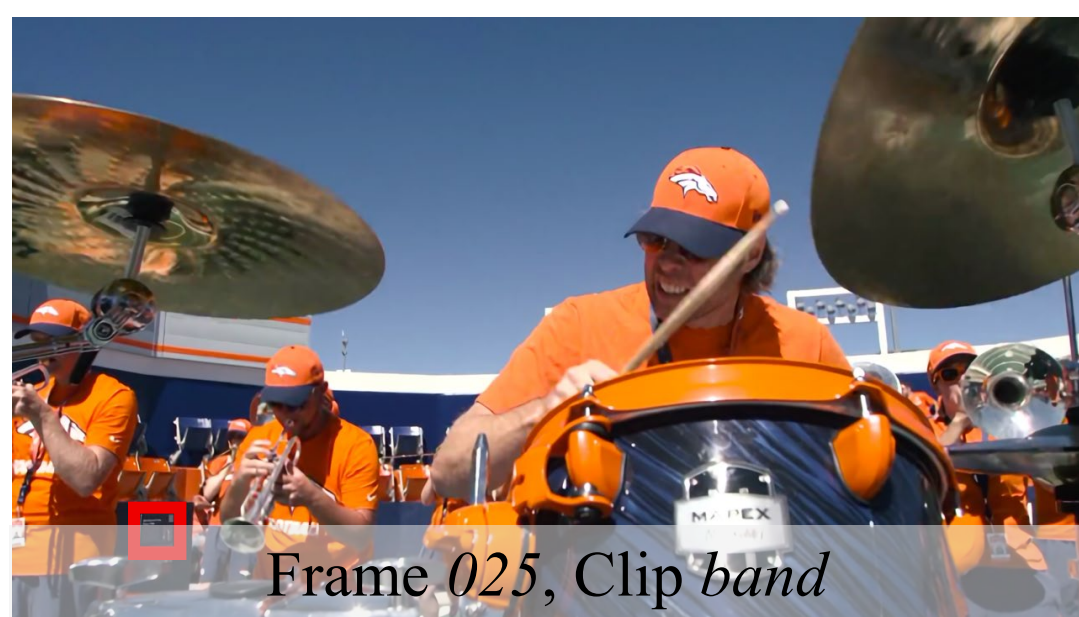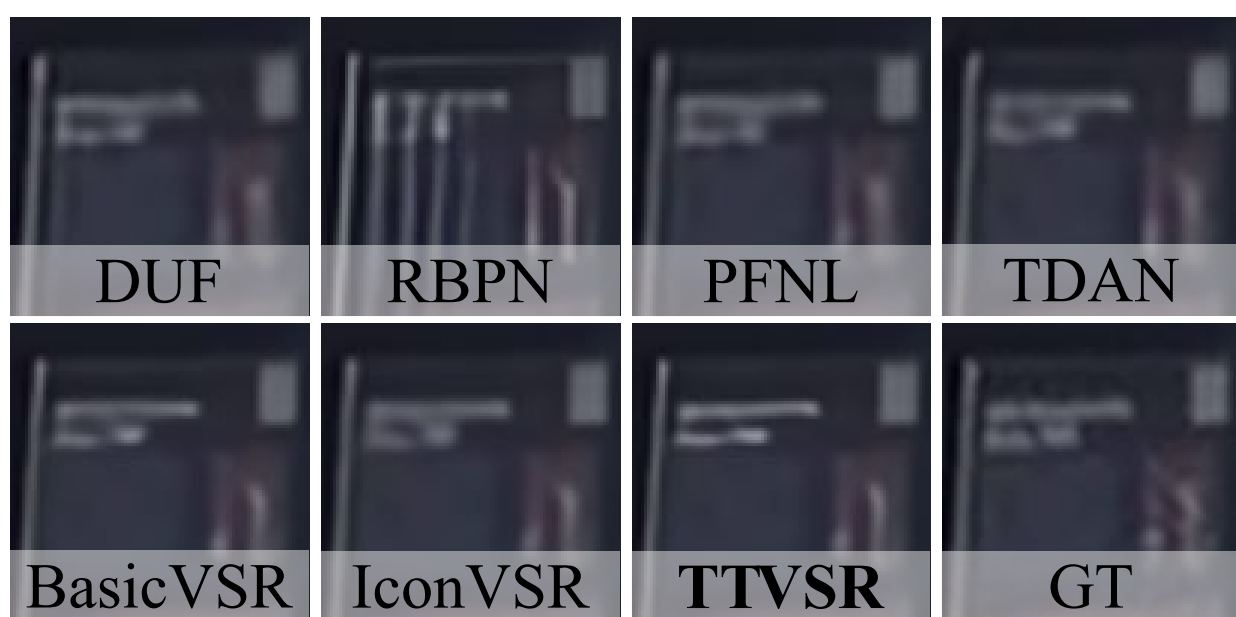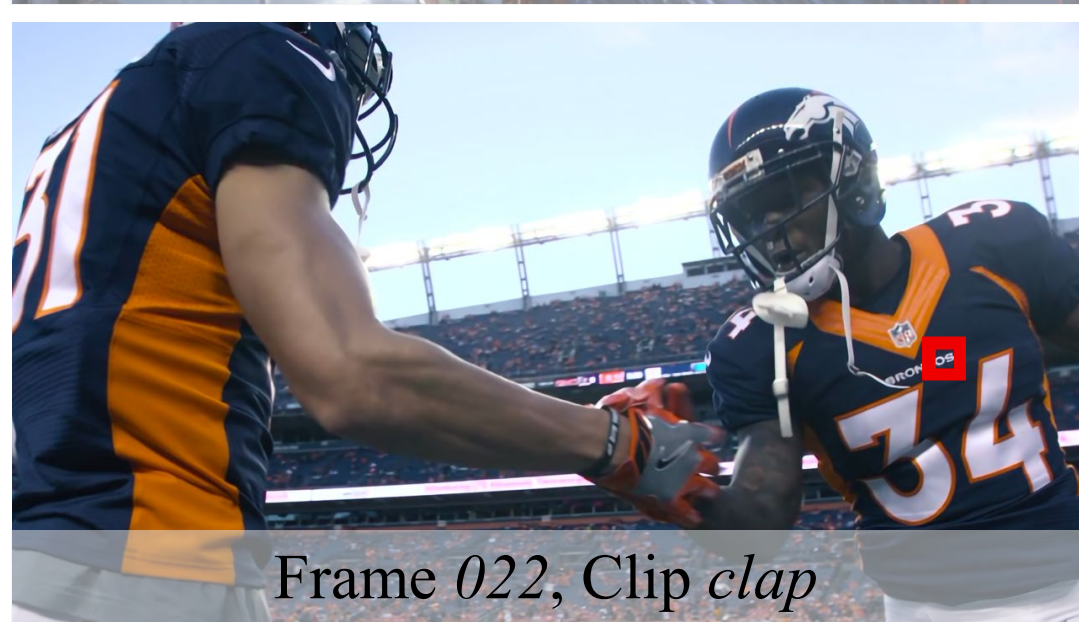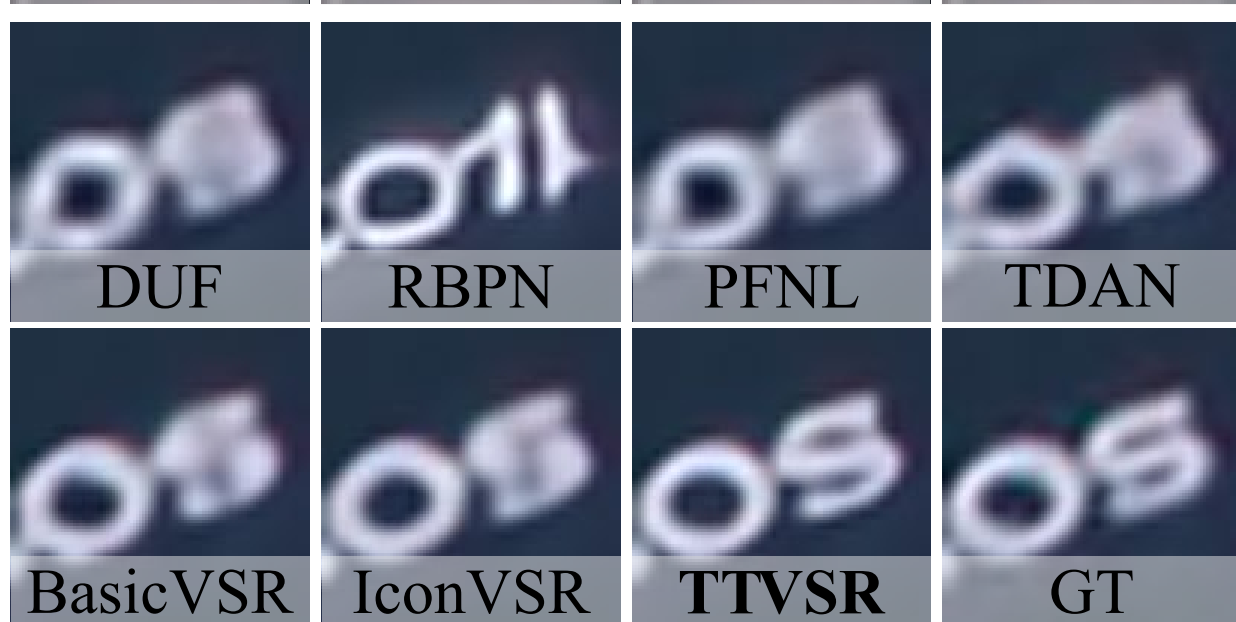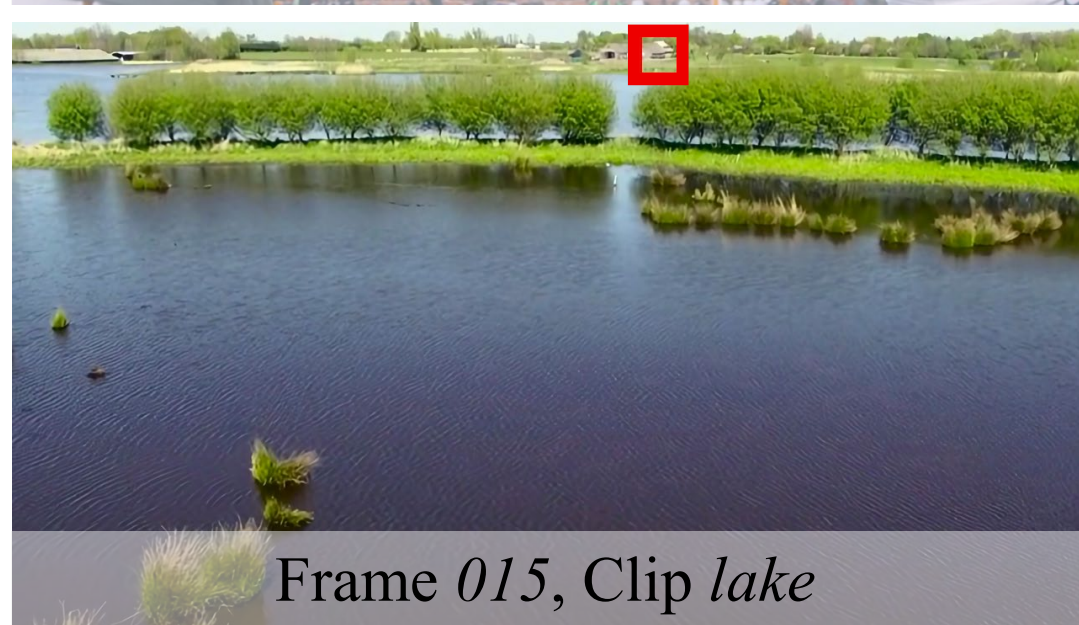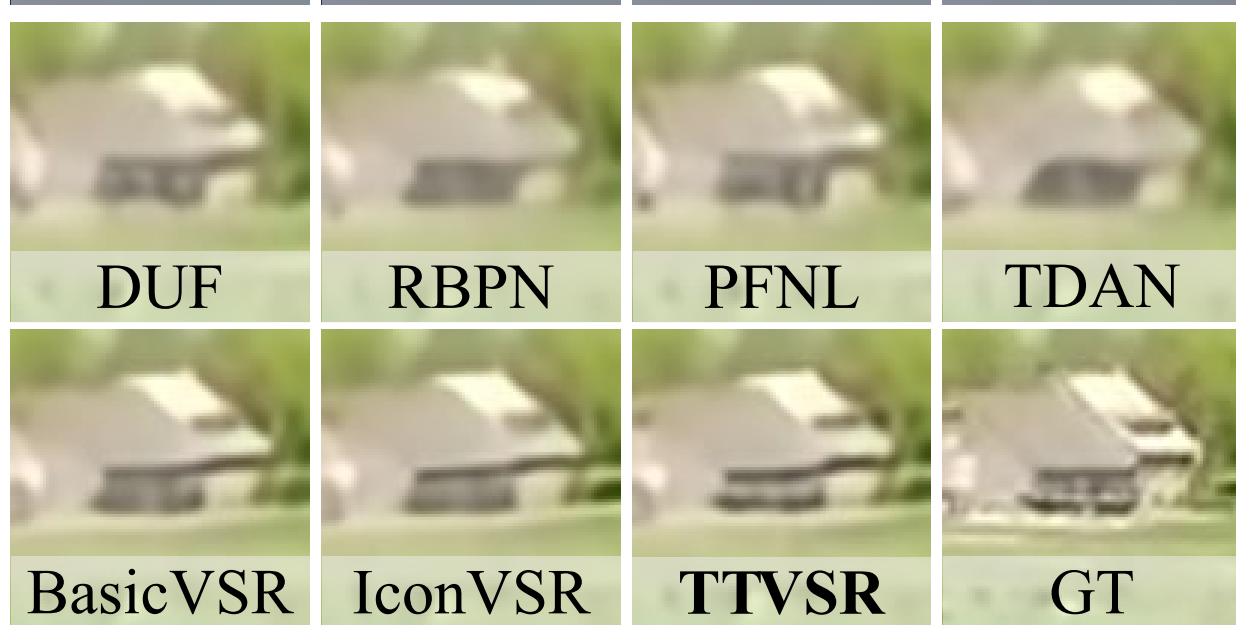



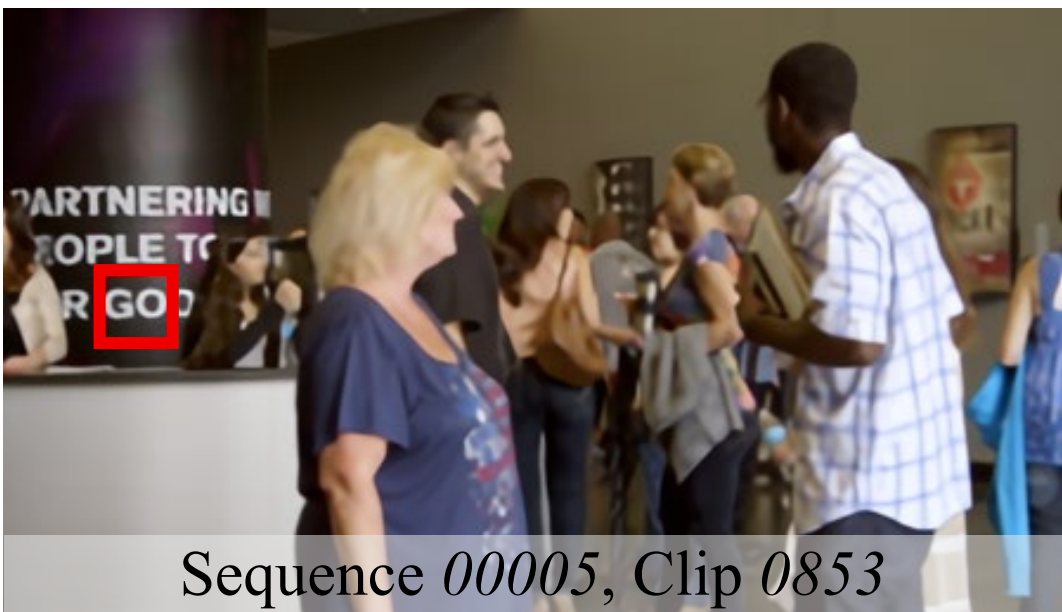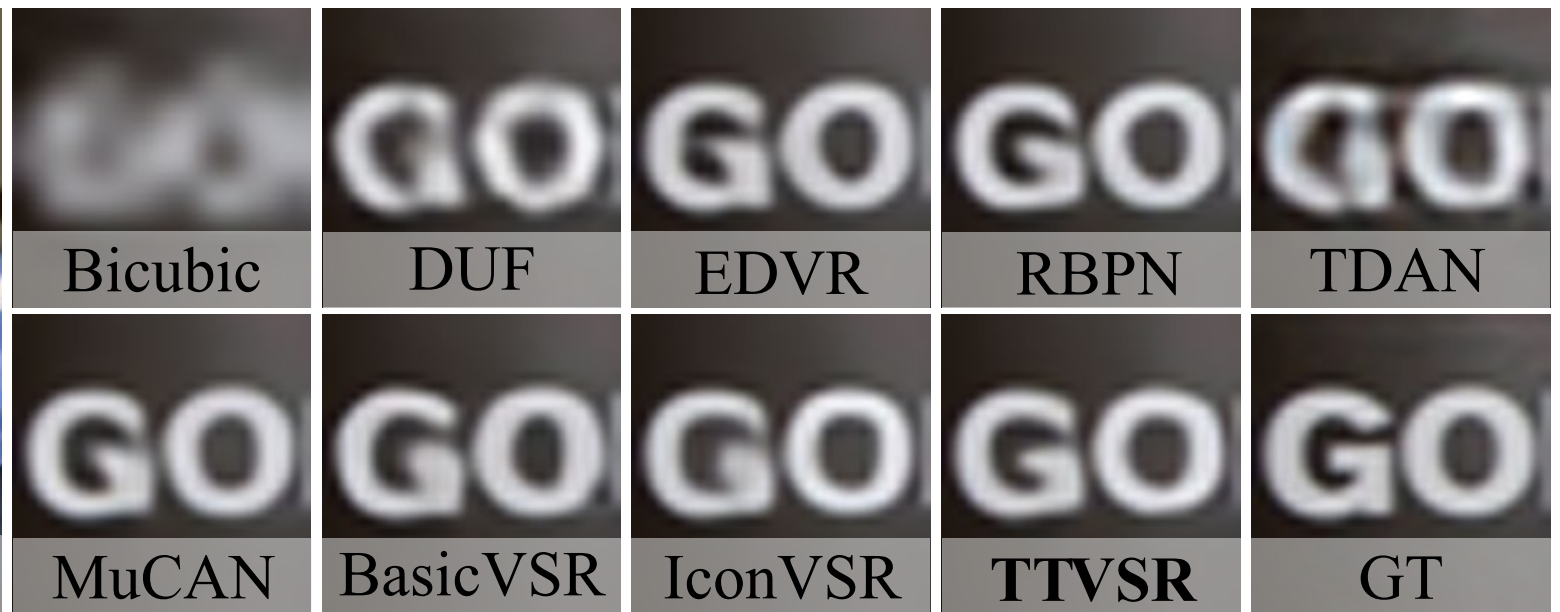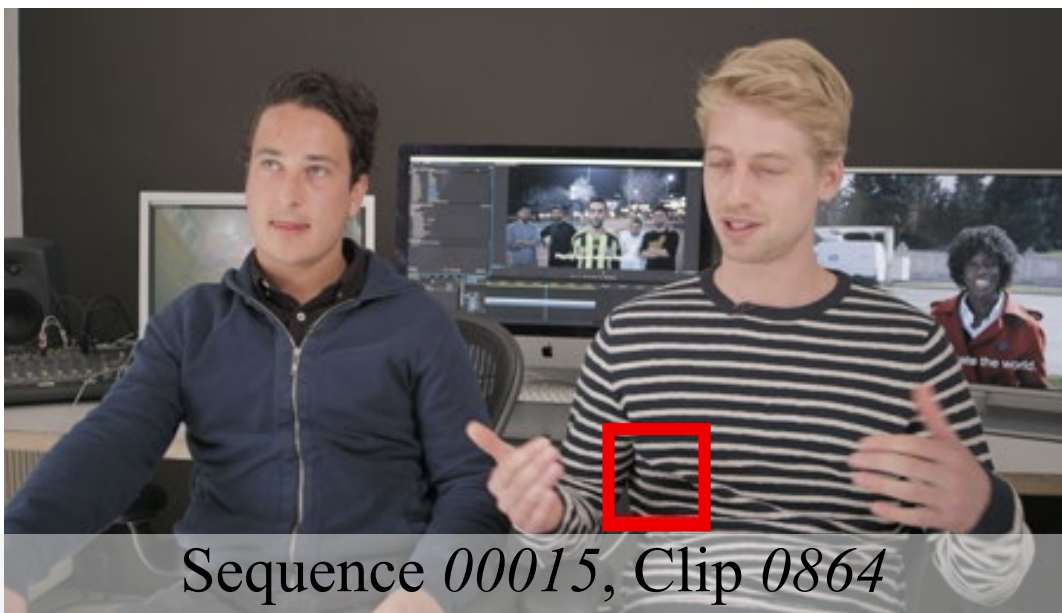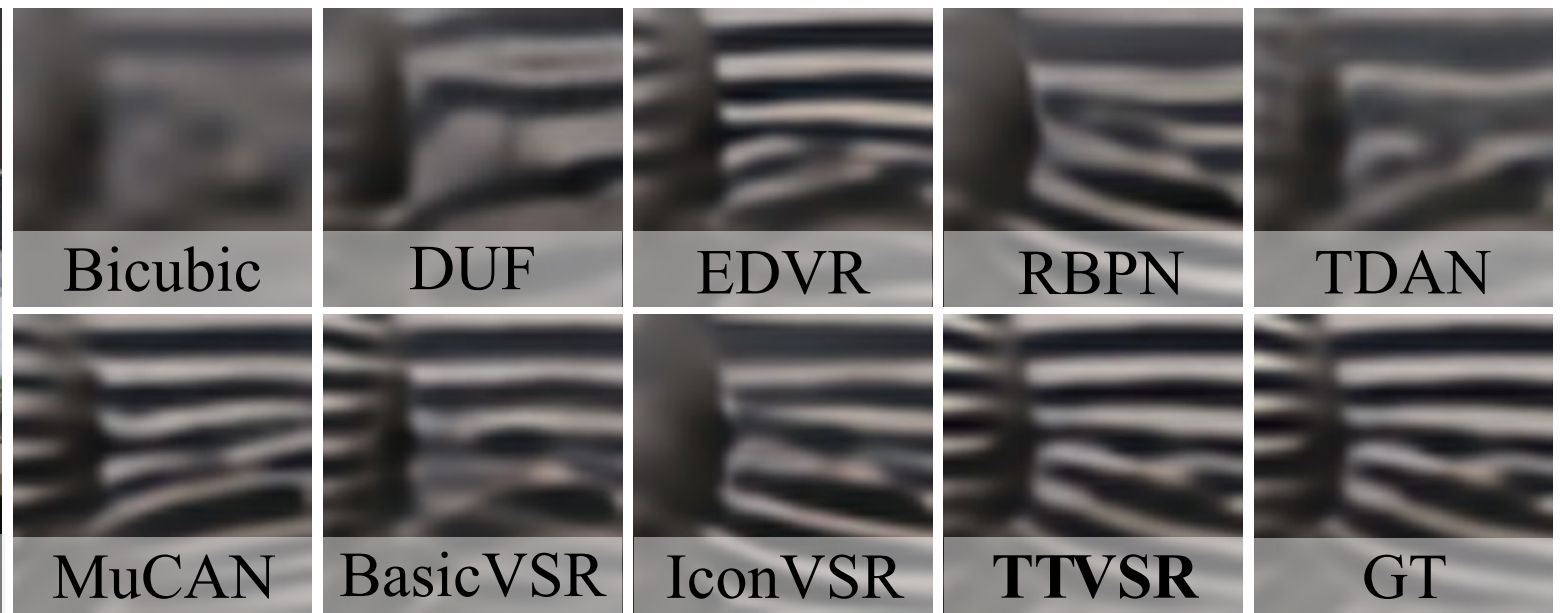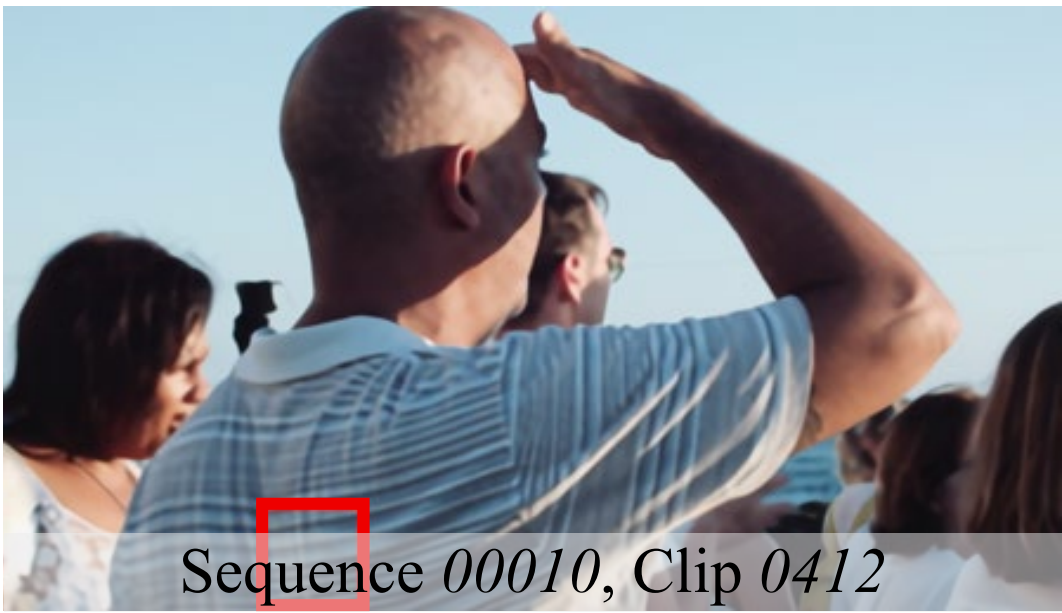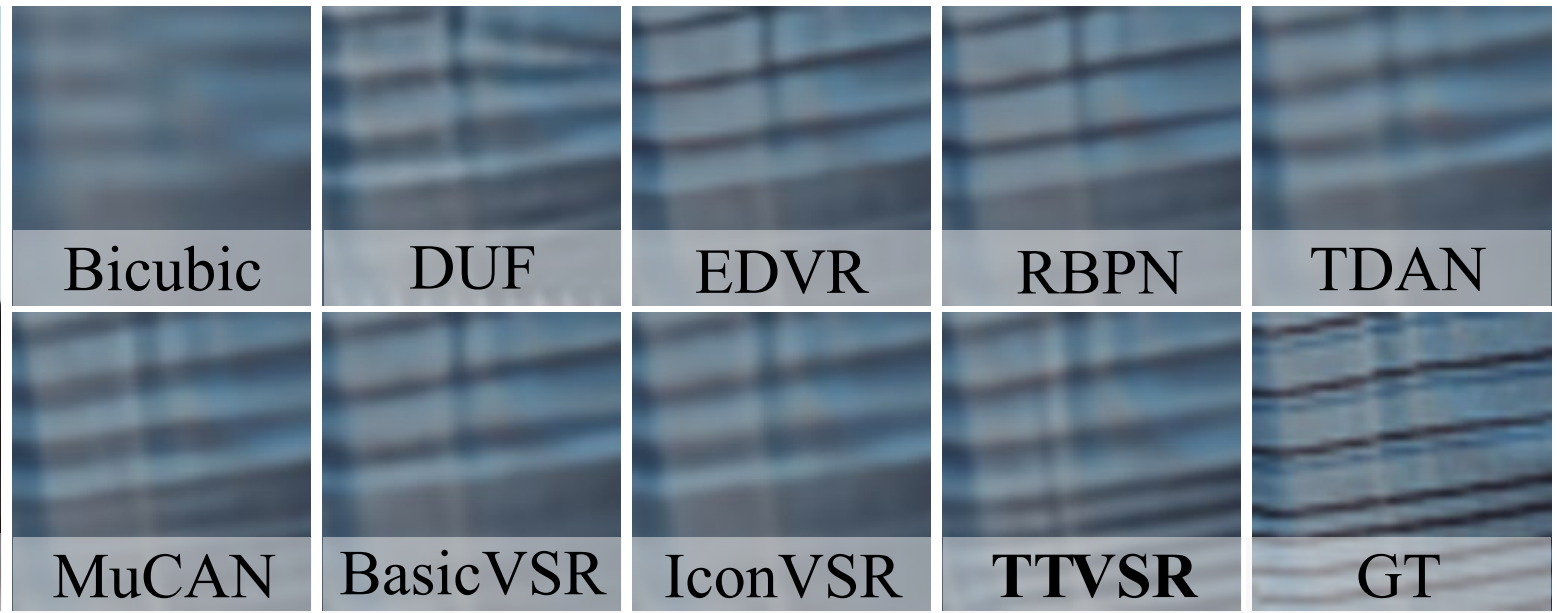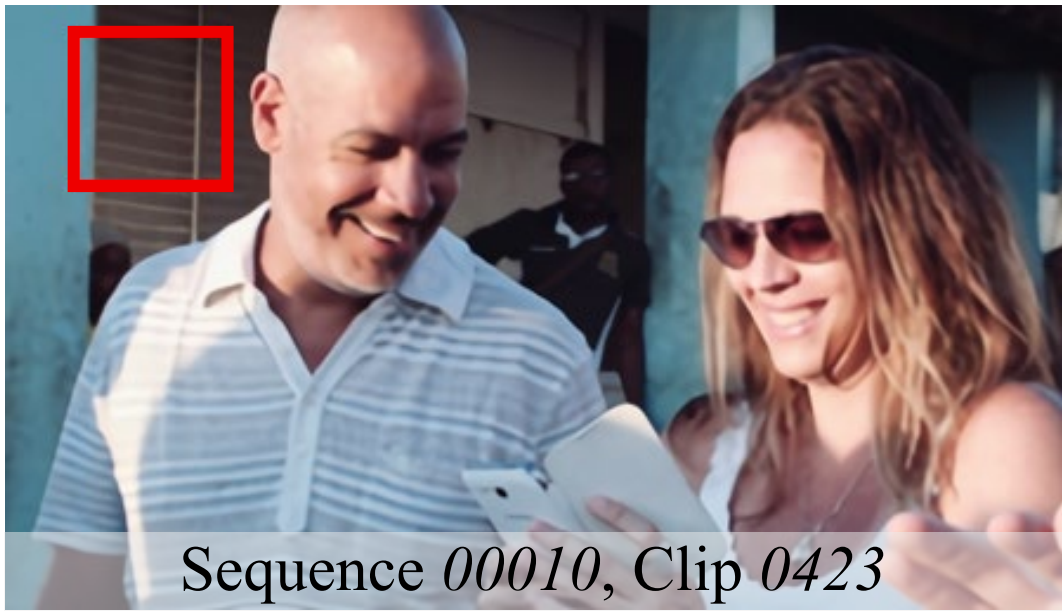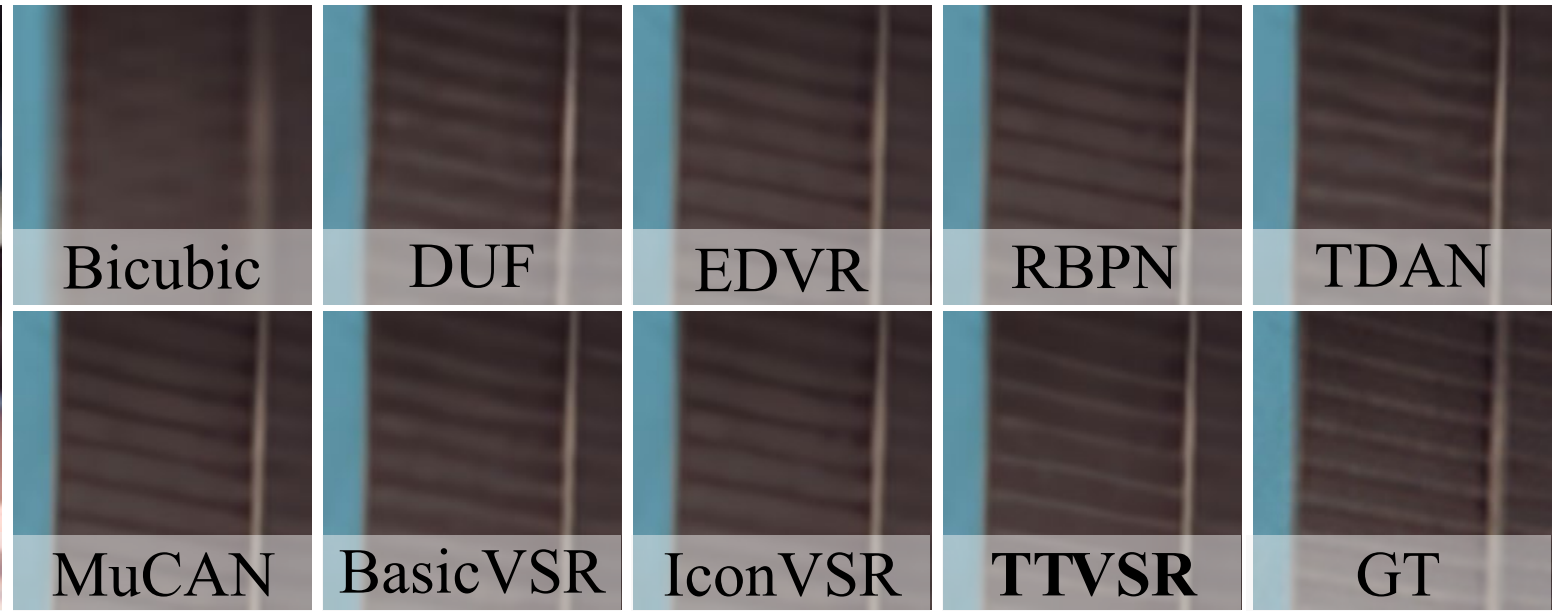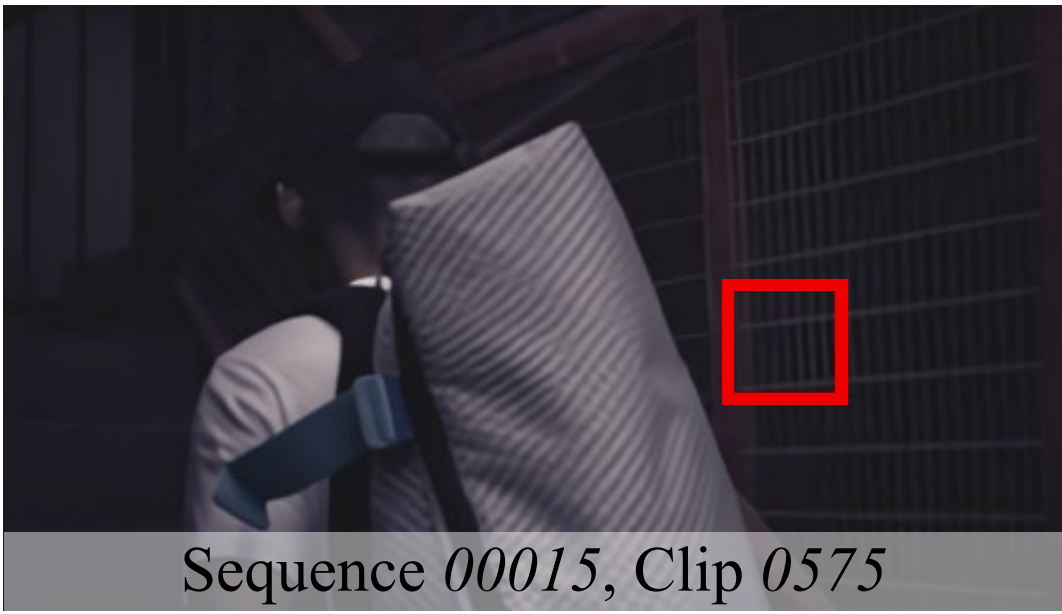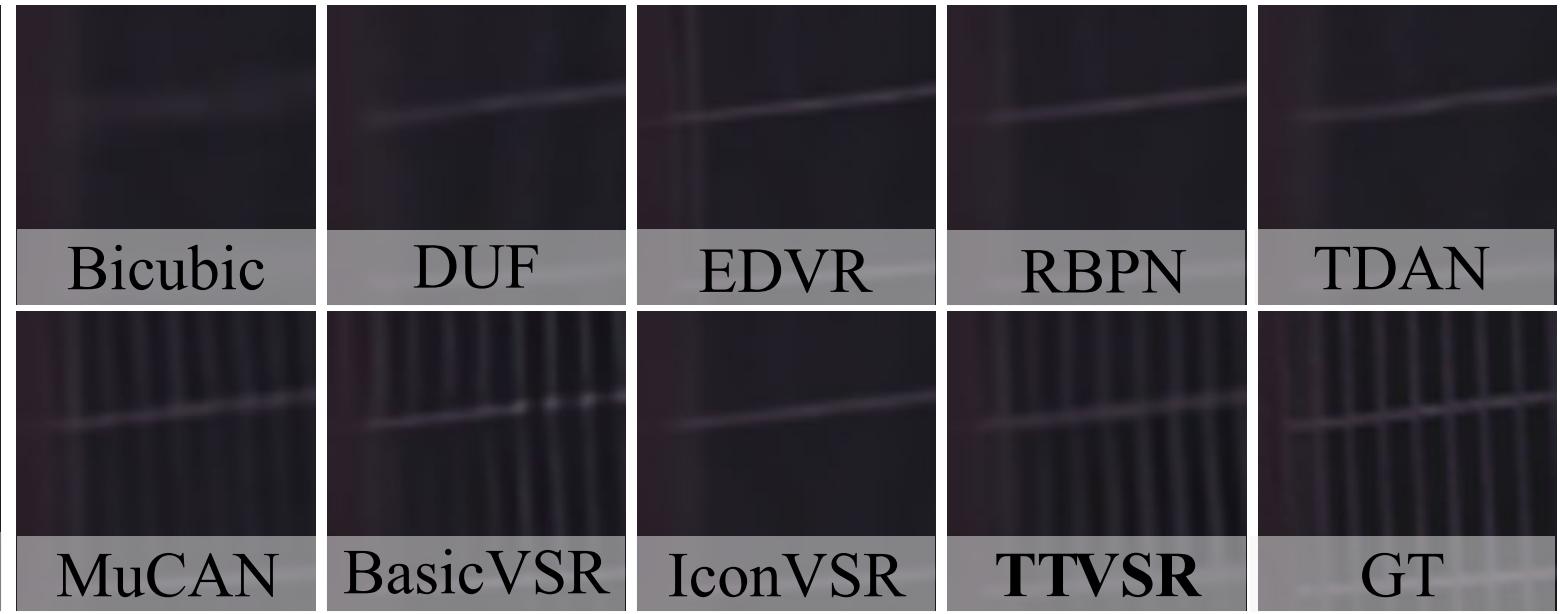



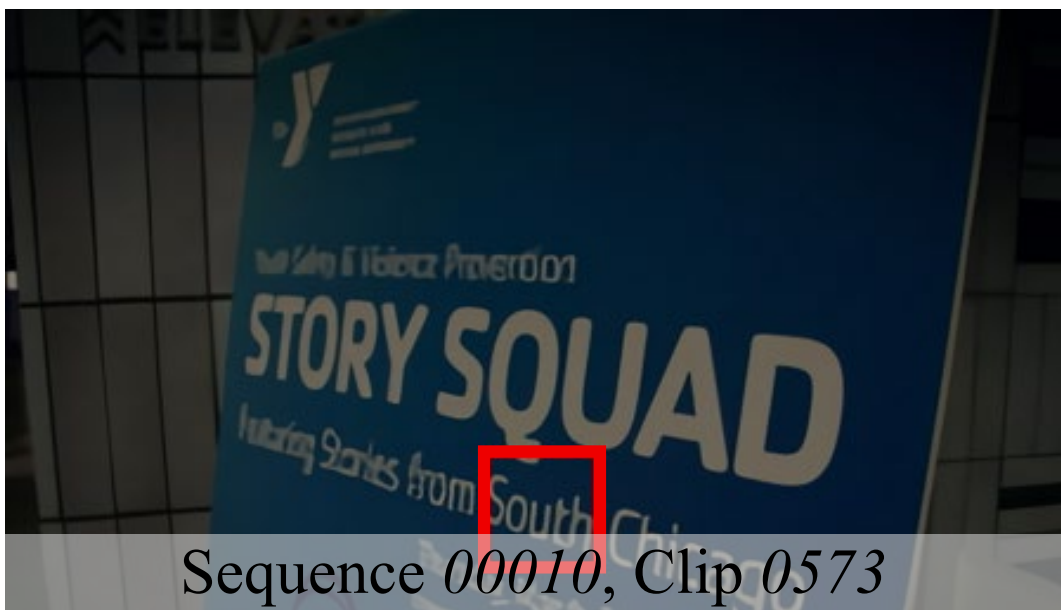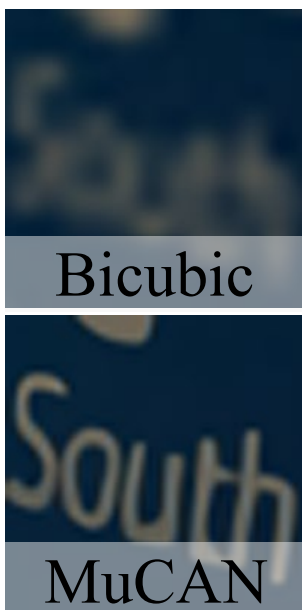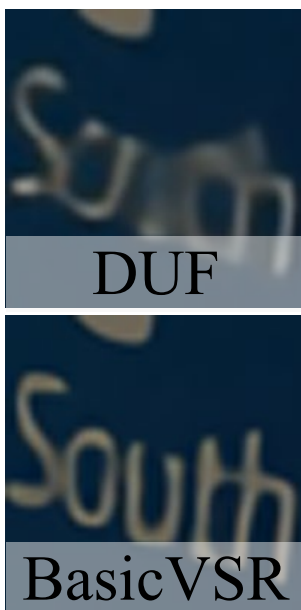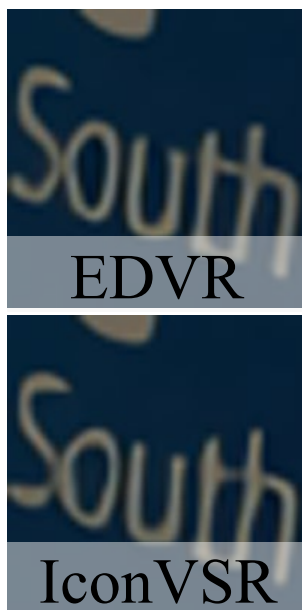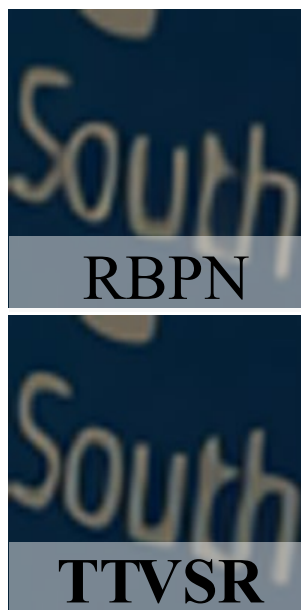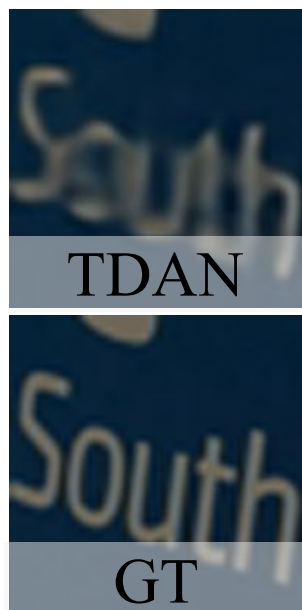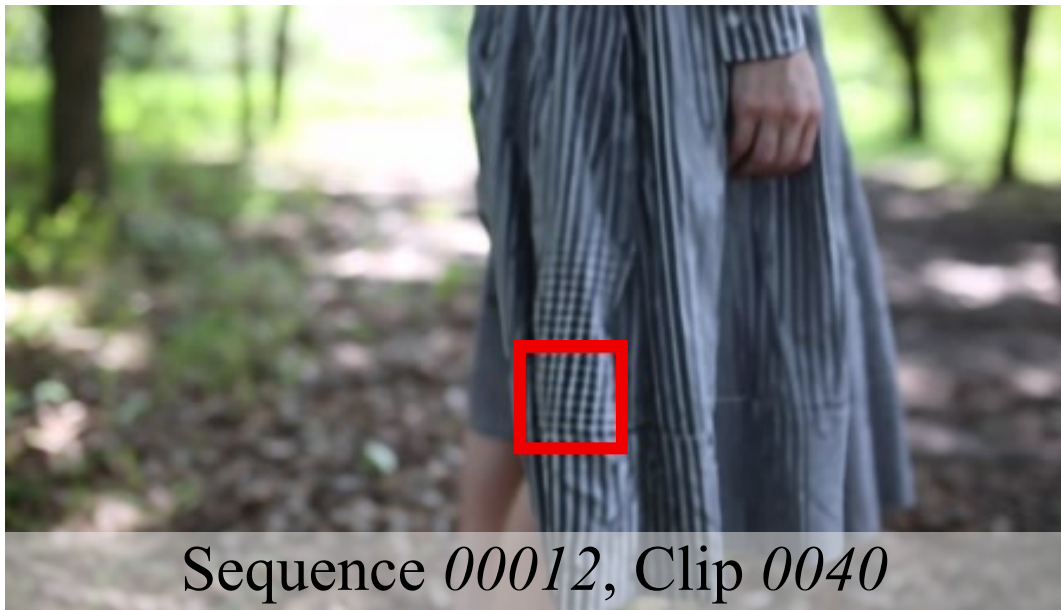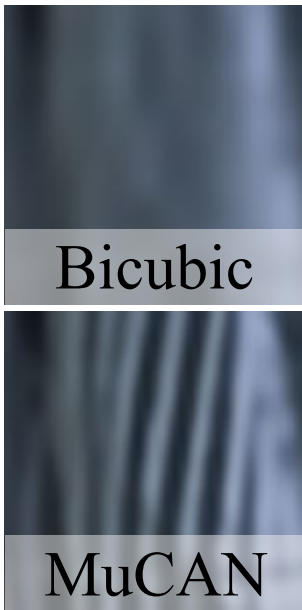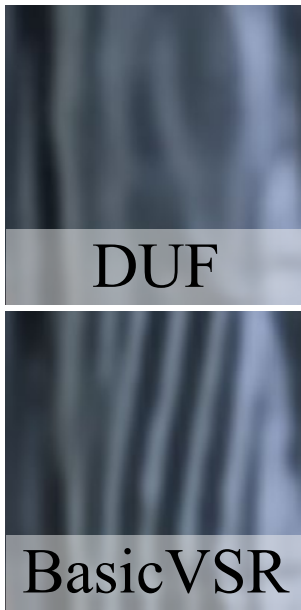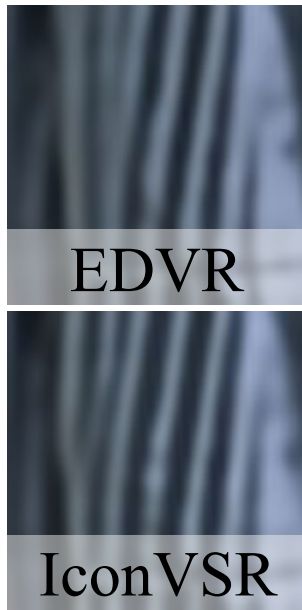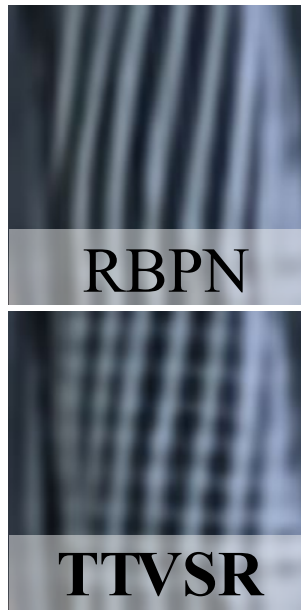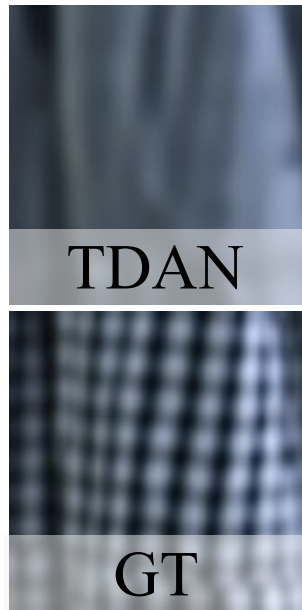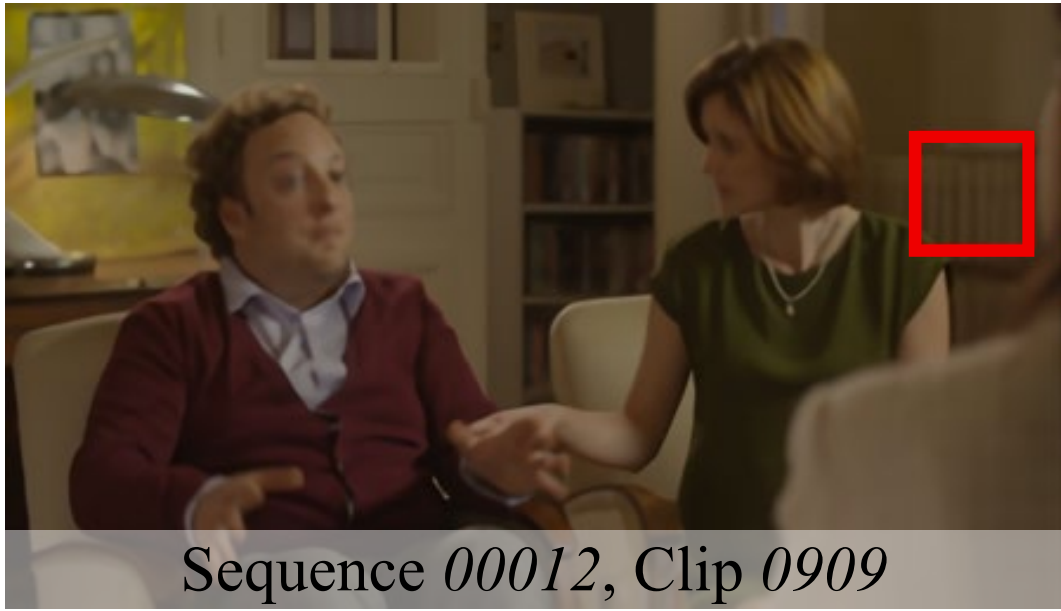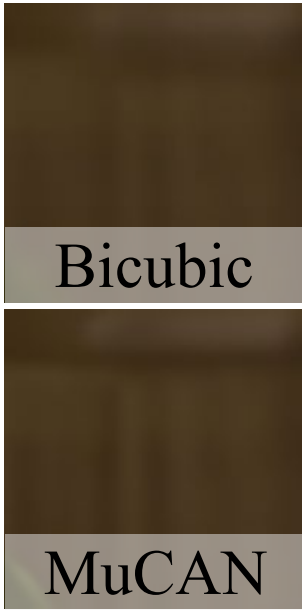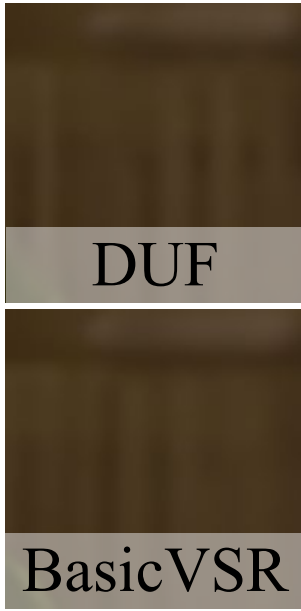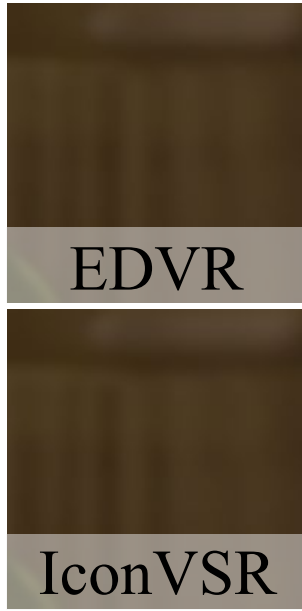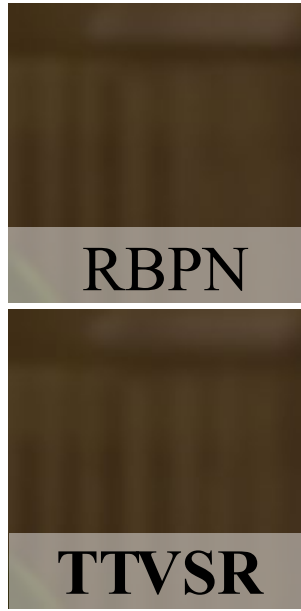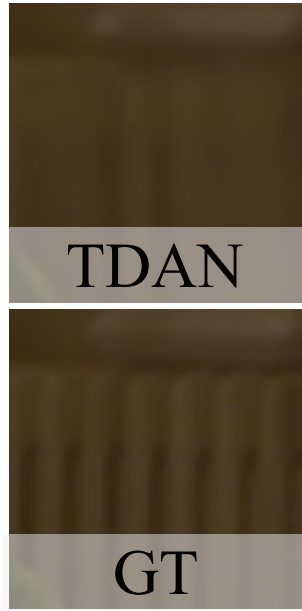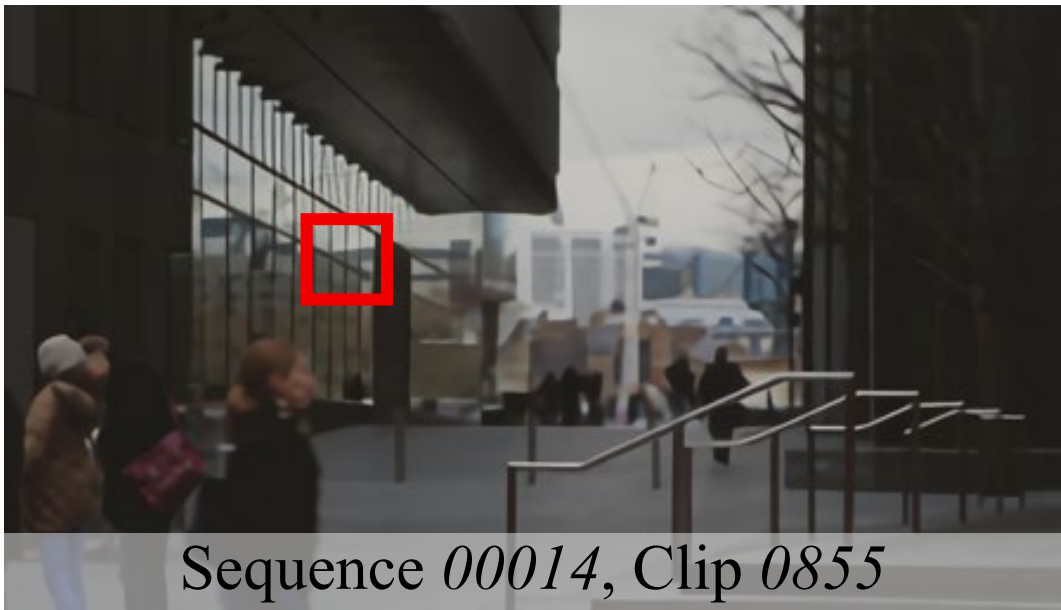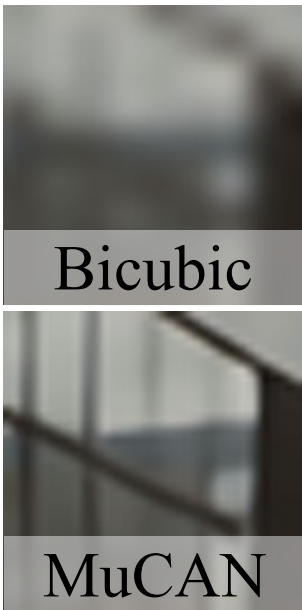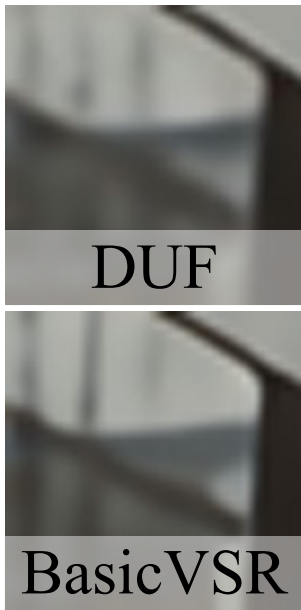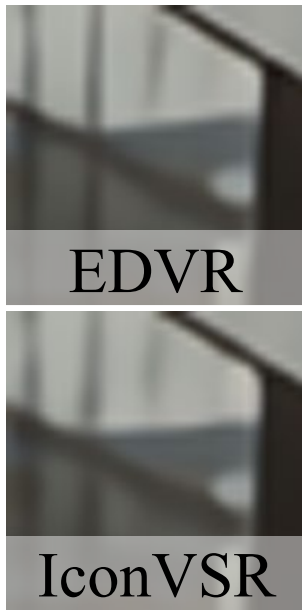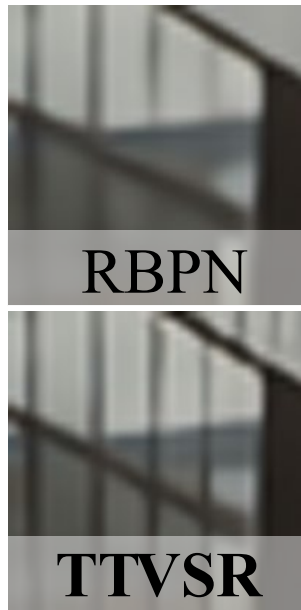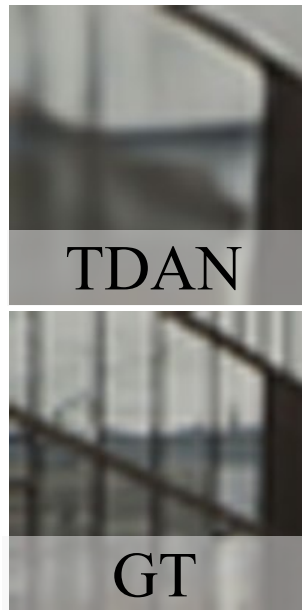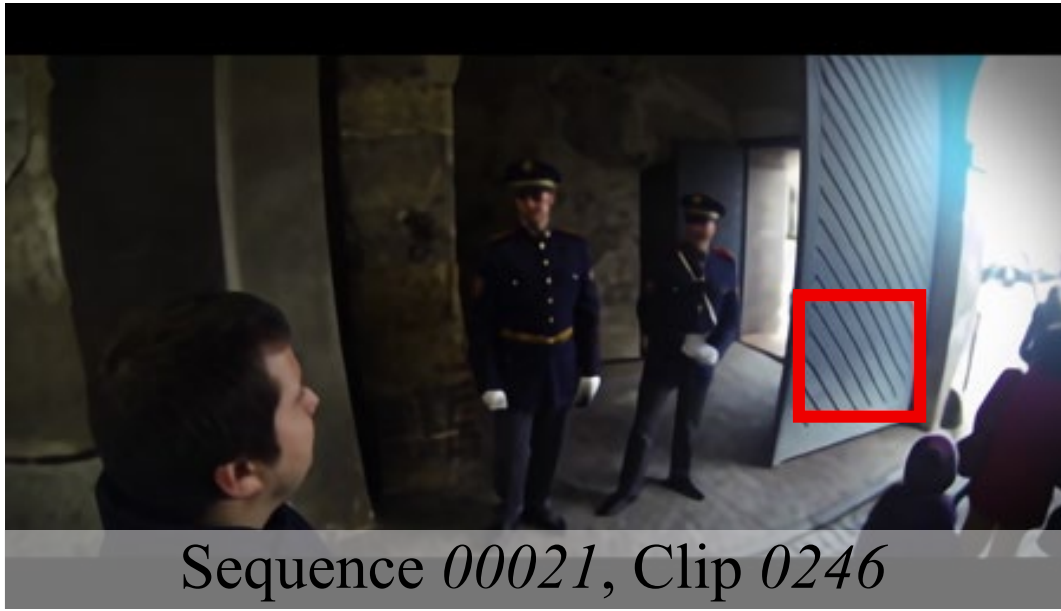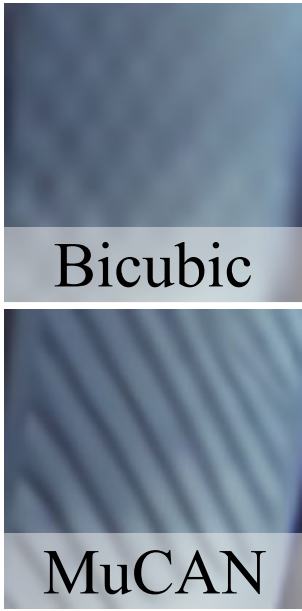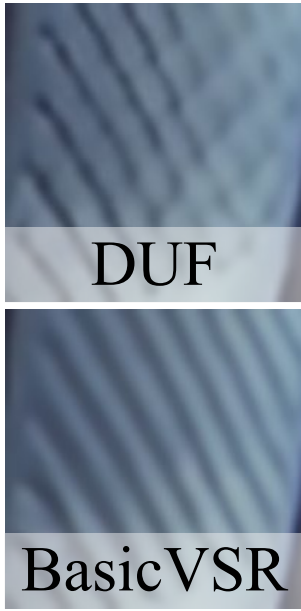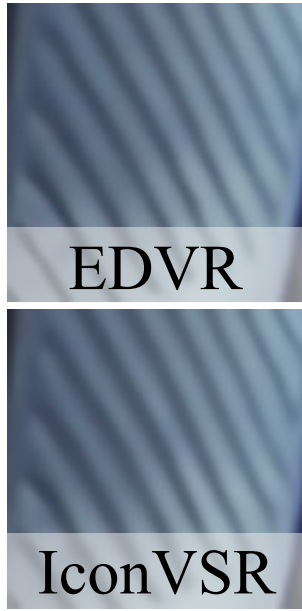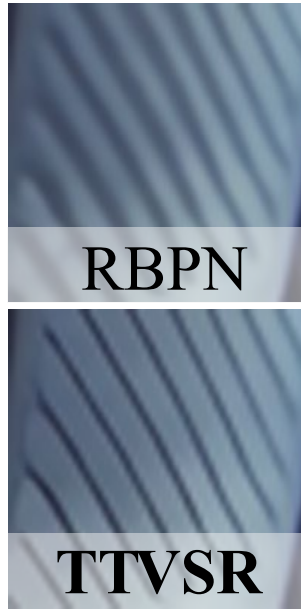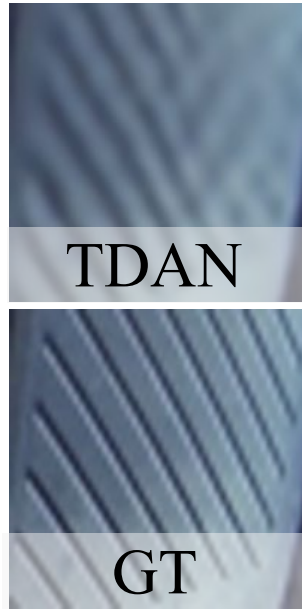

Supplement: Supplementary file 1 [file supplementary1_TTVSR.pdf]
